# Supplementary material for: New Implementation of an Equation-of-Motion Coupled-Cluster Damped-Response Framework with Illustrative Applications to Resonant Inelastic X-ray Scattering
Source: arXiv:2211.12215 source file (2023-01-19)
Supplement: Supplementary file 1 [file RIXS_SI.pdf]

# New Implementation of an Equation-of-Motion Coupled-Cluster Damped-Response Framework with Illustrative Applications to Resonant Inelastic X-ray Scattering. Supplementary Information

Anna Kristina Schnack-Petersen,[*,†] Torsha Moitra,[†,‡] Sarai Dery Folkestad,[¶] and Sonia Coriani[*,†,¶]

†*DTU Chemistry, Technical University of Denmark, DK-2800 Kongens Lyngby, Denmark*

‡*Hylleraas Centre for Quantum Molecular Sciences, Department of Chemistry, UiT – The Arctic University of Norway, 9037 Tromsø, Norway*

¶*Department of Chemistry, Norwegian University of Science and Technology, NO-7491 Trondheim, Norway*

E-mail: akrsc@kemi.dtu.dk; soco@kemi.dtu.dk

# S1 $H_2O$

Table S1: $H_2O$: Unshifted O *K*-edge XAS data using the 6-311++G** basis set with additional Rydberg functions on Oxygen.

| EOM-CC2 | | | EOM-CCSD | | | fc-EOM-CCSD | | |
|---|---|---|---|---|---|---|---|---|
| Sym.[a] | $\omega_{abs,c}$/eV | $f_{osc}$ | Sym.[a] | $\omega_{abs,c}$/eV | $f_{osc}$ | Sym.[b] | $\omega_{abs,c}$/eV | $f_{osc}$ |
| $1A_1$ | 534.4946 | 0.00615 | $1A_1$ | 535.6955 | 0.01179 | $1A_1$ | 535.2154 | 0.01266 |
| $1B_2$ | 536.0207 | 0.00834 | $1B_2$ | 537.4812 | 0.02512 | $1B_1$ | 537.0019 | 0.02607 |
| $1B_1$ | 536.5695 | 0.00155 | $1B_1$ | 538.9083 | 0.00558 | $1B_2$ | 538.4294 | 0.00596 |
| $2A_1$ | 536.6292 | 0.00077 | $2A_1$ | 539.0138 | 0.00443 | $2A_1$ | 538.5350 | 0.00454 |
| $3A_1$ | 536.7800 | 0.00167 | $3A_1$ | 539.3419 | 0.00161 | $3A_1$ | 538.8632 | 0.00169 |
| $2B_2$ | 537.1659 | 0.00299 | $2B_2$ | 539.6601 | 0.00522 | $2B_1$ | 539.1814 | 0.00552 |
| $2B_1$ | 537.3722 | 0.00054 | $2B_1$ | 540.2582 | 0.00181 | $2B_2$ | 539.7796 | 0.00189 |
| $4A_1$ | 537.3945 | 0.00031 | $4A_1$ | 540.2979 | 0.00156 | $4A_1$ | 539.8193 | 0.00160 |
| $5A_1$ | 537.4230 | 0.00053 | $5A_1$ | 540.3714 | 0.00043 | $5A_1$ | 539.8929 | 0.00045 |
| $3B_2$ | 537.6143 | 0.00222 | $3B_2$ | 540.4529 | 0.00134 | $3B_1$ | 539.9744 | 0.00142 |

[a] Dalton (Mulliken) symmetry notation.
[b] Q-Chem (non-Mulliken) symmetry notation.

Table S2: $H_2O$: Unshifted valence absorption data using the 6-311++G** basis set with additional Rydberg functions on Oxygen. In addition, valence transitions were computed in a space orthogonal to the oxygen core space.
[a] Dalton (Mulliken) symmetry notation. [b] Q-Chem (non-Mulliken) symmetry notation.

| EOM-CC2 | | | EOM-CCSD | | | fc-EOM-CCSD | | |
|---|---|---|---|---|---|---|---|---|
| Sym.[a] | $\omega_{abs,v}$/eV | $f_{osc}$ | Sym.[a] | $\omega_{abs,v}$/eV | $f_{osc}$ | Sym.[b] | $\omega_{abs,v}$/eV | $f_{osc}$ |
| $1B_1$ | 7.0638 | 0.04923 | $1B_1$ | 7.4049 | 0.04683 | $1B_2$ | 7.3824 | 0.04678 |
| $1A_2$ | 8.6920 | 0.00000 | $1A_2$ | 9.1558 | 0.00000 | $1A_2$ | 9.1349 | 0.00000 |
| $1A_1$ | 9.3046 | 0.03077 | $1A_1$ | 9.7566 | 0.08667 | $1A_1$ | 9.7348 | 0.08688 |
| $2B_1$ | 9.3881 | 0.00424 | $2B_1$ | 10.0254 | 0.00499 | $2B_2$ | 10.0055 | 0.00500 |
| $2A_1$ | 9.5193 | 0.06698 | $2A_1$ | 10.1116 | 0.01412 | $2A_1$ | 10.0917 | 0.01395 |
| $3B_1$ | 9.6651 | 0.00101 | $3B_1$ | 10.3876 | 0.00032 | $3B_2$ | 10.3675 | 0.00031 |
| $2A_2$ | 10.0870 | 0.00000 | $2A_2$ | 10.7960 | 0.00000 | $2A_2$ | 10.7760 | 0.00000 |
| $3A_1$ | 10.3722 | 0.00007 | $4B_1$ | 11.2175 | 0.00127 | $4B_2$ | 11.1980 | 0.00127 |
| $4B_1$ | 10.3802 | 0.00106 | $3A_1$ | 11.2220 | 0.00004 | $3A_1$ | 11.2026 | 0.00004 |
| $5B_1$ | 10.4456 | 0.00001 | $5B_1$ | 11.3052 | 0.00017 | $5B_2$ | 11.2857 | 0.00017 |
| $3A_2$ | 10.6127 | 0.00000 | $3A_2$ | 11.4226 | 0.00000 | $3A_2$ | 11.4030 | 0.00000 |
| $6B_1$ | 10.7838 | 0.00078 | $1B_2$ | 11.5198 | 0.02398 | $1B_1$ | 11.5000 | 0.02407 |
| $4A_1$ | 10.8119 | 0.00000 | $6B_1$ | 11.6806 | 0.00123 | $6B_2$ | 11.6612 | 0.00123 |
| $7B_1$ | 10.8396 | 0.00018 | $4A_1$ | 11.6957 | 0.00000 | $4A_1$ | 11.6764 | 0.00000 |
| $1B_2$ | 11.0385 | 0.01837 | $7B_1$ | 11.7220 | 0.00008 | $7B_2$ | 11.7026 | 0.00008 |
| $4A_2$ | 11.0468 | 0.00000 | $4A_2$ | 11.8183 | 0.00000 | $4A_2$ | 11.7987 | 0.00000 |
| $8B_1$ | 11.6090 | 0.00001 | $8B_1$ | 12.2254 | 0.00014 | $8B_2$ | 12.2063 | 0.00014 |
| $5A_1$ | 11.6434 | 0.00362 | $5A_1$ | 12.2847 | 0.00365 | $5A_1$ | 12.2657 | 0.00364 |
| $6A_1$ | 11.9789 | 0.01160 | $6A_1$ | 12.6793 | 0.01097 | $6A_1$ | 12.6597 | 0.01095 |

**Table S2 – continued from previous page**

| EOM-CC2 | | | EOM-CCSD | | | fc-EOM-CCSD | | |
|---|---|---|---|---|---|---|---|---|
| Sym.[a] | $\omega_{abs,v}$/eV | $f_{osc}$ | Sym.[a] | $\omega_{abs,v}$/eV | $f_{osc}$ | Sym.[b] | $\omega_{abs,v}$/eV | $f_{osc}$ |
| $2B_2$ | 12.4081 | 0.01235 | $9B_1$ | 13.0676 | 0.09370 | $9B_2$ | 13.0471 | 0.09350 |
| $9B_1$ | 12.6215 | 0.03281 | $2B_2$ | 13.1248 | 0.01858 | $5A_2$ | 13.1052 | 0.00000 |
| $7A_1$ | 12.6539 | 0.00116 | $5A_2$ | 13.1249 | 0.00000 | $2B_1$ | 13.1057 | 0.01861 |
| $10B_1$ | 12.6642 | 0.05516 | $10B_1$ | 13.4475 | 0.00034 | $10B_2$ | 13.4287 | 0.00033 |
| $5A_2$ | 12.6840 | 0.00000 | $7A_1$ | 13.4594 | 0.00093 | $7A_1$ | 13.4405 | 0.00092 |
| $8A_1$ | 12.7382 | 0.00361 | $11B_1$ | 13.5330 | 0.00896 | $11B_2$ | 13.5123 | 0.00902 |
| $3B_2$ | 12.9248 | 0.00991 | $8A_1$ | 13.5654 | 0.00350 | $8A_1$ | 13.5464 | 0.00349 |
| $9A_1$ | 13.0676 | 0.00008 | $3B_2$ | 13.7218 | 0.00666 | $3B_1$ | 13.7029 | 0.00669 |
| $11B_1$ | 13.0808 | 0.00016 | $9A_1$ | 13.8849 | 0.00012 | $9A_1$ | 13.8654 | 0.00012 |
| $10A_1$ | 13.1174 | 0.00390 | $4B_2$ | 13.9215 | 0.14358 | $4B_1$ | 13.9038 | 0.14340 |
| $12B_1$ | 13.1320 | 0.00927 | $12B_1$ | 13.9299 | 0.00002 | $12B_2$ | 13.9112 | 0.00002 |
| $4B_2$ | 13.3851 | 0.02269 | $10A_1$ | 13.9741 | 0.00276 | $10A_1$ | 13.9553 | 0.00275 |
| $11A_1$ | 13.5834 | 0.00177 | $11A_1$ | 14.04896 | 0.00175 | $5B_1$ | 14.1122 | 0.06424 |
| $5B_2$ | 13.6877 | 0.16906 | $5B_2$ | 14.13095 | 0.06400 | $6A_2$ | 14.7908 | 0.00000 |

Table S3: $H_2O$: Unshifted RIXS data for the pump frequency at resonance with the first core excitation (core $1A_1$) calculated using different methods. RIXS cross sections for $\theta = 45°$ at the EOM-CCSD, CVS-uS-EOM-CCSD and CVS-EOM-CCSD level of theory are all based on emission energies calculated at the EOM-CCSD level of theory. CVS and CVS-uS refer to a projection in the damped response solver. All calculations employed the 6-311++G** basis set with additional Rydberg functions on Oxygen.

| $\omega_{em}$/eV | | | $\sigma^{\mathrm{RIXS}}_{45°}$/a.u. | | | | |
|---|---|---|---|---|---|---|---|
| CCSD | fc-CCSD | CC2 | EOM-CCSD | CVS-uS-EOM-CCSD | CVS-EOM-CCSD | fc-CVS-EOM-CCSD | EOM-CC2 |
| 528.2906 | 527.8331 | 527.4307 | 0.02113 | 0.02152 | 0.01928 | 0.02107 | 0.01259 |
| 526.5398 | 526.0807 | 525.8026 | 0.00040 | 0.00040 | 0.00034 | 0.00016 | 0.00038 |
| 525.9389 | 525.4821 | 525.1898 | 0.01162 | 0.01218 | 0.01067 | 0.01156 | 0.00244 |
| 525.6701 | 525.2100 | 525.1065 | 0.00063 | 0.00056 | 0.00032 | 0.00005 | 0.00055 |
| 525.5838 | 525.1229 | 524.9754 | 0.00210 | 0.00222 | 0.00231 | 0.00207 | 0.00606 |
| 525.3079 | 524.848 | 524.8295 | 0.00023 | 0.00024 | 0.00021 | 0.00023 | 0.00002 |
| 524.8995 | 524.4399 | 524.4075 | 0.00002 | 0.00001 | 0.00000 | 0.00003 | 0.00001 |
| 524.4780 | 524.0181 | 524.1223 | 0.00013 | 0.00012 | 0.00006 | 0.00001 | 0.00002 |
| 524.4736 | 524.0127 | 524.1144 | 0.00002 | 0.00002 | 0.00014 | 0.00002 | 0.00012 |
| 524.3903 | 523.931 | 524.0491 | 0.00005 | 0.00006 | 0.00005 | 0.00005 | 0.00000 |
| 524.2728 | 523.8113 | 523.8818 | 0.00003 | 0.00003 | 0.00000 | 0.00001 | 0.00001 |
| 524.1756 | 523.7160 | 523.7109 | 0.00035 | 0.00037 | 0.00086 | 0.00012 | 0.00005 |
| 524.0148 | 523.5555 | 523.6826 | 0.00007 | 0.00007 | 0.00004 | 0.00001 | 0.00001 |
| 523.9999 | 523.5392 | 523.6551 | 0.00000 | 0.00000 | 0.00010 | 0.00000 | 0.00009 |
| 523.9735 | 523.5120 | 523.4559 | 0.00006 | 0.00006 | 0.00003 | 0.00001 | 0.00031 |
| 523.8771 | 523.4167 | 523.4477 | 0.00011 | 0.00011 | 0.00003 | 0.00000 | 0.00014 |
| 523.4701 | 523.0086 | 522.8856 | 0.00046 | 0.00046 | 0.00023 | 0.00001 | 0.00043 |
| 523.4107 | 522.9487 | 522.8513 | 0.00011 | 0.00011 | 0.00021 | 0.00007 | 0.00007 |
| 523.0162 | 522.5568 | 522.5158 | 0.00018 | 0.00018 | 0.00017 | 0.00018 | 0.00001 |
| 522.6279 | 522.1677 | 522.0866 | 0.00020 | 0.00023 | 0.00018 | 0.00017 | 0.00003 |
| 522.5707 | 522.1106 | 521.8730 | 0.00005 | 0.00005 | 0.00012 | 0.00004 | 0.00017 |
| 522.5704 | 522.1106 | 521.8406 | 0.00020 | 0.00018 | 0.00005 | 0.00000 | 0.00001 |
| 522.2480 | 521.7868 | 521.8303 | 0.00010 | 0.00010 | 0.00005 | 0.00000 | 0.00000 |
| 522.2360 | 521.7759 | 521.8104 | 0.00001 | 0.00001 | 0.00007 | 0.00001 | 0.00026 |
| 522.1625 | 521.7024 | 521.7563 | 0.00083 | 0.00074 | 0.00032 | 0.00004 | 0.00000 |
| 522.1302 | 521.6697 | 521.5699 | 0.00003 | 0.00003 | 0.00004 | 0.00003 | 0.00002 |
| 521.9737 | 521.5119 | 521.4270 | 0.00031 | 0.00033 | 0.00032 | 0.00033 | 0.00000 |
| 521.8107 | 521.3514 | 521.4137 | 0.00001 | 0.00001 | 0.00025 | 0.00001 | 0.00009 |
| 521.774 | 521.3106 | 521.3772 | 0.01381 | 0.01449 | 0.01303 | 0.01429 | 0.00000 |
| 521.7655 | 521.3051 | 521.3625 | 0.00007 | 0.00007 | 0.00003 | 0.00000 | 0.00086 |
| | | 521.1095 | | | | | 0.00008 |
| | | 520.9111 | | | | | 0.00002 |
| | | 520.8069 | | | | | 0.00877 |

Table S4: $H_2O$: unshifted RIXS data for the pump frequency at resonance with the second core excitation (core $1B_2$ in Mulliken symmetry notation) calculated using different methods. RIXS cross sections for $\theta = 45^\circ$ at the EOM-CCSD, CVS-uS-EOM-CCSD and CVS-EOM-CCSD level of theory are all based on emission energies calculated at the EOM-CCSD level of theory. CVS and CVS-uS refers to a projection in the damped response solver. All calculations employed the 6-311++G** basis set with additional Rydberg functions on Oxygen.

| $\omega_{em}$/eV | | | $\sigma^{\mathrm{RIXS}}_{45^\circ}$/a.u. | | | | |
|---|---|---|---|---|---|---|---|
| CCSD | fc-CCSD | CC2 | EOM-CCSD | CVS-uS-EOM-CCSD | CVS-EOM-CCSD | fc-CVS-EOM-CCSD | EOM-CC2 |
| 530.0764 | 529.6182 | 528.9570 | 0.00007 | 0.00006 | 0.00004 | 0.00013 | 0.00005 |
| 528.3254 | 527.8658 | 527.3286 | 0.04099 | 0.04192 | 0.03876 | 0.04067 | 0.01648 |
| 527.7246 | 527.2671 | 526.7161 | 0.00010 | 0.00011 | 0.00020 | 0.00010 | 0.00012 |
| 527.4560 | 526.9950 | 526.6326 | 0.00063 | 0.00060 | 0.00037 | 0.00003 | 0.00074 |
| 527.3697 | 526.9107 | 526.5014 | 0.00017 | 0.00018 | 0.00072 | 0.00022 | 0.00009 |
| 527.0935 | 526.6331 | 526.3556 | 0.00000 | 0.00000 | 0.00001 | 0.00001 | 0.00010 |
| 526.6851 | 526.2249 | 525.9338 | 0.00188 | 0.00195 | 0.00179 | 0.00188 | 0.00010 |
| 526.2639 | 525.8032 | 525.6486 | 0.00012 | 0.00012 | 0.00007 | 0.00000 | 0.00001 |
| 526.2592 | 525.8004 | 525.6404 | 0.00005 | 0.00005 | 0.00020 | 0.00005 | 0.00012 |
| 526.1760 | 525.7161 | 525.5751 | 0.00000 | 0.00000 | 0.00000 | 0.00000 | 0.00000 |
| 526.0587 | 525.5991 | 525.4081 | 0.00052 | 0.00056 | 0.00050 | 0.00053 | 0.00001 |
| 525.9615 | 525.5011 | 525.2369 | 0.03230 | 0.03327 | 0.02982 | 0.03103 | 0.00006 |
| 525.8007 | 525.3406 | 525.2089 | 0.00005 | 0.00005 | 0.00004 | 0.00000 | 0.00001 |
| 525.7855 | 525.3242 | 525.1811 | 0.00003 | 0.00003 | 0.00014 | 0.00003 | 0.00008 |
| 525.7591 | 525.2998 | 524.9822 | 0.00005 | 0.00005 | 0.00002 | 0.00000 | 0.01365 |
| 525.6630 | 525.2018 | 524.9738 | 0.00031 | 0.00036 | 0.00027 | 0.00025 | 0.00012 |
| 525.2559 | 524.7963 | 524.4118 | 0.00064 | 0.00062 | 0.00036 | 0.00005 | 0.00077 |
| 525.1966 | 524.7365 | 524.3773 | 0.00011 | 0.00012 | 0.00029 | 0.00012 | 0.00004 |
| 524.8021 | 524.3419 | 524.0418 | 0.00005 | 0.00005 | 0.00005 | 0.00003 | 0.00010 |
| 524.4135 | 523.9555 | 523.6126 | 0.00007 | 0.00007 | 0.00001 | 0.00001 | 0.00008 |
| 524.3563 | 523.8956 | 523.3993 | 0.00217 | 0.00218 | 0.00191 | 0.00194 | 0.00017 |
| 524.3563 | 523.8956 | 523.3669 | 0.00027 | 0.00030 | 0.00017 | 0.00012 | 0.00000 |
| 524.0339 | 523.5718 | 523.3566 | 0.00012 | 0.00012 | 0.00006 | 0.00001 | 0.00000 |
| 524.0219 | 523.5609 | 523.3367 | 0.00001 | 0.00001 | 0.00008 | 0.00001 | 0.00025 |
| 523.9482 | 523.4902 | 523.2826 | 0.00075 | 0.00071 | 0.00031 | 0.00001 | 0.00001 |
| 523.9158 | 523.4548 | 523.0959 | 0.00000 | 0.00000 | 0.00002 | 0.00000 | 0.00003 |
| 523.7593 | 523.2997 | 522.9530 | 0.00083 | 0.00083 | 0.00070 | 0.00073 | 0.00000 |
| 523.5963 | 523.1364 | 522.9400 | 0.00034 | 0.00036 | 0.00059 | 0.00035 | 0.00010 |
| 523.5599 | 523.0983 | 522.9032 | 0.00008 | 0.00008 | 0.00004 | 0.00009 | 0.00000 |
| 523.5514 | 523.0902 | 522.8888 | 0.00008 | 0.00008 | 0.00004 | 0.00000 | 0.00089 |
| | | 522.6355 | | | | | 0.00004 |
| | | 522.4374 | | | | | 0.00035 |
| | | 522.3332 | | | | | 0.00004 |

Table S5: $H_2O$: Unshifted nonresonant (XES) data calculated using different methods. All calculations employed the 6-311++G** basis set with additional Rydberg functions on Oxygen.

| $\omega_{em}$/eV | | | $f_{osc}$ | | |
|---|---|---|---|---|---|
| CCSD | fc-CCSD | CC2 | EOM-CCSD | fc-CVS-EOM-CCSD | EOM-CC2 |
| 529.1262 | 528.6672 | 526.7877 | 0.05311 | 0.05361 | 0.05556 |
| 526.8753 | 526.4157 | 524.5019 | 0.04308 | 0.04359 | 0.04459 |
| 522.5313 | 522.0673 | 519.981 | 0.03881 | 0.03938 | 0.04028 |

### S1.1 Valence Transition NTOs

| EOM-CCSD | | | EOM-CC2 | | |
|---|---|---|---|---|---|
| Transition Symmetry | Hole NTO | Particle NTO | Transition Symmetry | Hole NTO | Particle NTO |
| $1B_1$ | 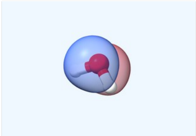 | 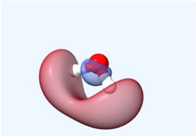 | $1B_1$ | 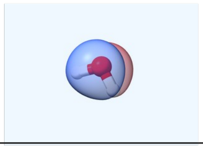 | 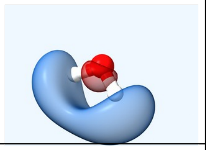 |
| $1A_2$ | 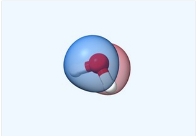 | 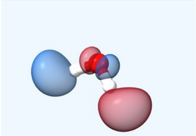 | $1A_2$ | 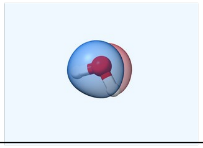 | 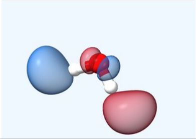 |
| $1A_1$ | 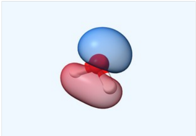 | 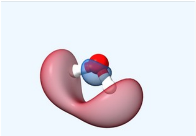 | $1A_1$ | 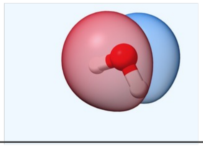 | 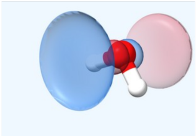 |
| $2A_1$ | 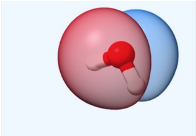 | 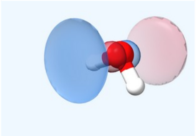 | $2A_1$ | 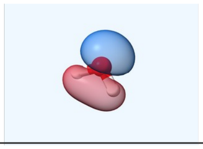 | 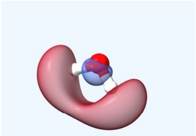 |
| $1B_2$ | 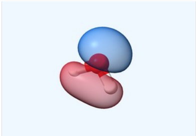 | 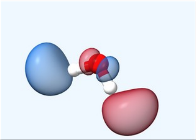 | $1B_2$ | 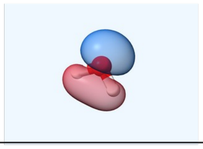 | 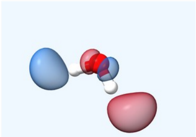 |
| $4B_2$ | 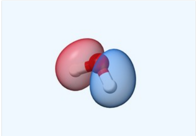 | 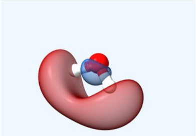 | $5B_2$ | 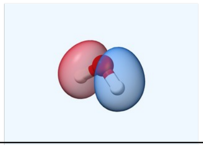 | 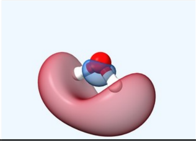 |

Figure S1: $H_2O$: NTO pairs of the probed valence transitions at both the CCSD and CC2 levels of theory. Isosurface value was 0.02-0.05 for all NTO pairs.

## S2 $CH_3OH$

XAS spectra at both carbon and oxygen *K*-edge were computed at the CVS-EOM-CCSD and the CVS-EOM-CC2 levels of theory, and they are shown in Fig. S2. At the O *K*-edge (left panels of Fig. S2), there are some noticeable differences between CC2 and CCSD, in particular in the position of the second transition as well as in the overall intensity of the XAS spectrum. The differences are somewhat smaller for the C *K*-edge XAS spectra, where the CVS-EOM-CC2 results

show a second peak with lower intensity and a third peak of higher intensity compared to both the CVS-EOM-CCSD result and experiment. For both methods the separation between the first transition and the second (intense) band is smaller than in the experiment. The first two transitions are of $A'$ symmetry at both levels of theory at the Oxygen $K$-edge. Likewise, both methods yield the first core transition at the Carbon $K$-edge to have $A'$ symmetry. Observe that all the plotted core excitations are below the calculated ionization thresholds. Prince et al.[1] assigned the higher

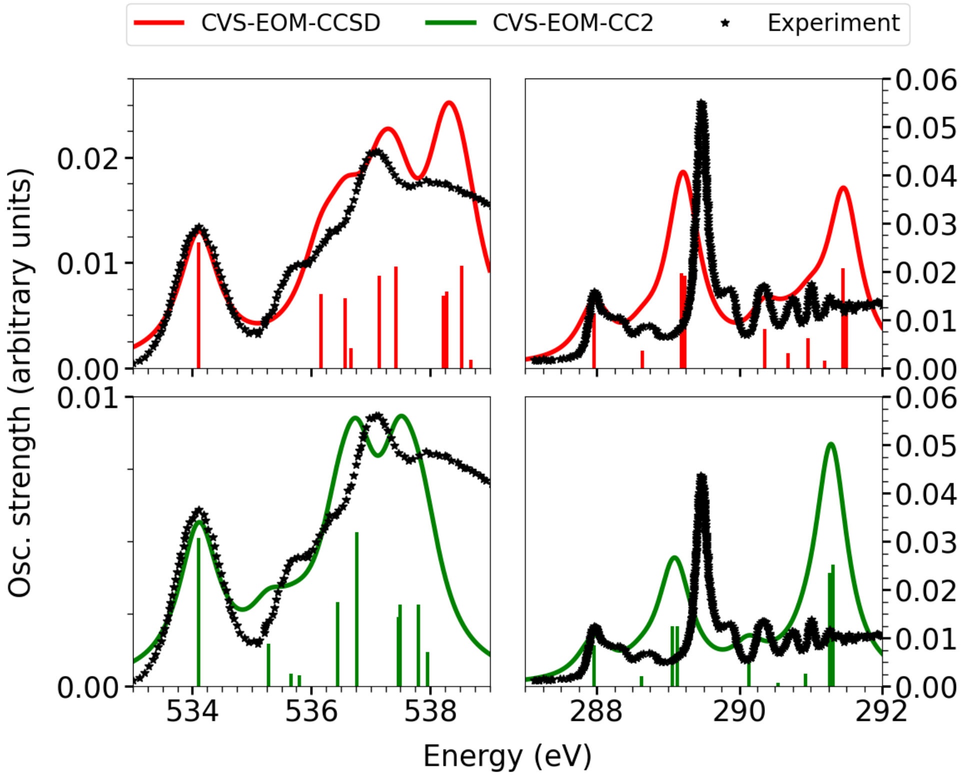


Figure S2: $CH_3OH$: XAS spectra at the Oxygen (left) and Carbon (right) $K$-edge calculated at the CVS-EOM-CC2/aug-cc-pVTZ (green) and CVS-EOM-CCSD/aug-cc-pVTZ (red) levels of theory. In both cases 10 core transitions were determined and plotted. The experimental data (black) was adapted from Prince et al.[1] A Lorentzian broadening was applied with HWHM=0.41 eV for O $K$-edge and HWHM=0.27 eV for C $K$-edge. At the O $K$-edge, the CVS-EOM-CCSD result was shifted by 0.07 eV to align with experiment, while the CVS-EOM-CC2 result was shifted by $-1.39$ eV. At the C $K$-edge, the shifts were $-2.09$ eV and $-1.07$ eV, respectively

energy experimental features at the C $K$-edge mainly to vibrational states, but also to some extent to more diffuse orbitals as, e.g., $5p$ and $6p$. These features are not reproduced by our calculations. Improvements might be obtained by including more diffuse functions in the basis set, however,

the features caused by vibrations would still be beyond such calculations. As our main concern is the first few strong features, we content ourselves with the chosen levels of theory as these show reasonable agreement for this region. We observe that the valence spectra in Fig. S3 are very

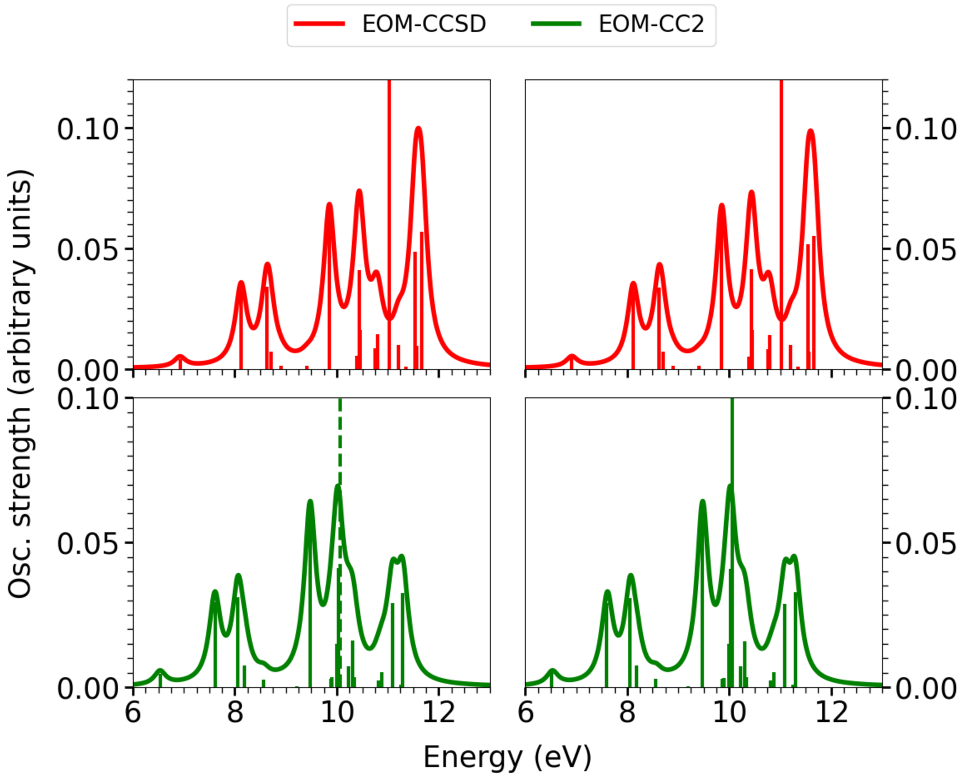


Figure S3: $CH_3OH$: Valence absorption spectra calculated in the space orthogonal to the O core space (left) or the C core space (right). The calculations employed the CVS-EOM-CC2/aug-cc-pVTZ level of theory (green) and the CVS-EOM-CCSD/aug-cc-pVTZ level of theory (red). In both cases, 20 valence transitions were determined and plotted. The first valence ionization energies are shown as vertical lines spanning the entire intensity. Results have been shifted to match the EOM-CCSD results computed in a space orthogonal to the O core space. A Lorentzian broadening has been applied with HWHM=0.41 eV.

similar for the two methods, except for a small difference in the shifts between the three peaks at lowest energy. The valence spectra are practically unaffected by changing which core space should be orthogonal to the space employed for the calculation.

#### S2.0.1 Data tables

Table S6: $CH_3OH$: Unshifted XAS data calculated with the aug-cc-pVTZ basis.

| Oxygen $K$-edge | | | | | | Carbon $K$-edge | | | | | |
|---|---|---|---|---|---|---|---|---|---|---|---|
| | EOM-CC2 | | | EOM-CCSD | | | EOM-CC2 | | | EOM-CCSD | |
| Sym.[a] | $\omega_{abs,c}$/eV | $f_{osc}$ | Sym.[a] | $\omega_{abs,c}$/eV | $f_{osc}$ | Sym.[a] | $\omega_{abs,c}$/eV | $f_{osc}$ | Sym.[a] | $\omega_{abs,c}$/eV | $f_{osc}$ |
| $1A'$ | 534.0381 | 0.00512 | $1A'$ | 535.4971 | 0.01195 | $1A'$ | 290.0519 | 0.00838 | $1A'$ | 289.0359 | 0.01128 |
| $2A'$ | 535.2052 | 0.00146 | $2A'$ | 537.5454 | 0.00699 | $2A'$ | 290.7113 | 0.00213 | $2A'$ | 289.7148 | 0.00348 |
| $1A''$ | 535.5883 | 0.00043 | $3A'$ | 537.9517 | 0.00663 | $1A''$ | 291.1412 | 0.01245 | $1A''$ | 290.2563 | 0.01956 |
| $3A'$ | 535.7216 | 0.00038 | $1A''$ | 538.0538 | 0.00186 | $3A'$ | 291.2186 | 0.01251 | $3A'$ | 290.3097 | 0.01906 |
| $4A'$ | 536.3741 | 0.00290 | $4A'$ | 538.5324 | 0.00877 | $4A'$ | 292.2152 | 0.00567 | $4A'$ | 291.4261 | 0.00799 |
| $5A'$ | 536.6930 | 0.00533 | $5A'$ | 538.8164 | 0.00959 | $5A'$ | 292.6274 | 0.00070 | $5A'$ | 291.7484 | 0.00299 |
| $2A''$ | 537.3881 | 0.00238 | $2A''$ | 539.6072 | 0.00687 | $6A'$ | 293.0101 | 0.00259 | $A2''$ | 292.0348 | 0.00617 |
| $6A'$ | 537.4183 | 0.00283 | $6A'$ | 539.6603 | 0.00723 | $2A''$ | 293.0729 | 0.00001 | $6A'$ | 292.2661 | 0.00151 |
| $7A'$ | 537.7288 | 0.00281 | $7A'$ | 539.9127 | 0.00971 | $A3''$ | 293.3538 | 0.02341 | $7A'$ | 292.5199 | 0.02069 |
| $8A'$ | 537.8811 | 0.00118 | $8A'$ | 540.0707 | 0.00078 | $7A'$ | 293.3934 | 0.02527 | $3A''$ | 292.5698 | 0.01331 |

[a] Mulliken symmetry notation.

Table S7: $CH_3OH$: Unshifted valence absorption data computed in a space orthogonal to the core space (with a "removed core" projector) and aug-cc-pVTZ basis on all atoms.

| Oxygen as "removed core" | | | | | | Carbon as "removed core" | | | | | |
|---|---|---|---|---|---|---|---|---|---|---|---|
| | EOM-CC2 | | | EOM-CCSD | | | EOM-CC2 | | | EOM-CCSD | |
| Sym.[a] | $\omega_v$/eV | $f_{osc}$ | Sym.[a] | $\omega_{abs,v}$/eV | $f_{osc}$ | Sym.[a] | $\omega_{abs,v}$/eV | $f_{osc}$ | Sym.[a] | $\omega_{abs,v}$/eV | $f_{osc}$ |
| $1A''$ | 6.5321 | 0.00473 | $1A''$ | 6.9241 | 0.00415 | $1A''$ | 6.5205 | 0.00486 | $1A''$ | 6.9128 | 0.00427 |
| $2A''$ | 7.6093 | 0.02929 | $2A''$ | 8.1227 | 0.03225 | $2A''$ | 7.6017 | 0.02902 | $2A''$ | 8.1168 | 0.03193 |
| $1A'$ | 8.0627 | 0.03106 | $1A'$ | 8.6336 | 0.03401 | $1A'$ | 8.0548 | 0.03088 | $A1'$ | 8.6270 | 0.03384 |
| $3A''$ | 8.1923 | 0.00737 | $3A''$ | 8.7071 | 0.00699 | $3A''$ | 8.1838 | 0.00737 | $3A''$ | 8.6998 | 0.00700 |
| $2A'$ | 8.5677 | 0.00252 | $2A'$ | 8.9076 | 0.00122 | $2A'$ | 8.5585 | 0.00273 | $2A'$ | 8.8999 | 0.00137 |
| $4A''$ | 8.8868 | 0.00011 | $4A''$ | 9.4176 | 0.00130 | $4A''$ | 8.8766 | 0.00010 | $4A''$ | 9.4083 | 0.00126 |
| $5A''$ | 9.2134 | 0.00024 | $5A''$ | 9.7079 | 0.00000 | $5A''$ | 9.2022 | 0.00025 | $5A''$ | 9.6978 | 0.00000 |
| $3A'$ | 9.4778 | 0.05852 | $3A'$ | 9.8547 | 0.06272 | $3A'$ | 9.4735 | 0.05814 | $3A'$ | 9.8532 | 0.06236 |
| $4A'$ | 9.8817 | 0.00282 | $4A'$ | 10.4000 | 0.00548 | $4A'$ | 9.8718 | 0.00275 | $4A'$ | 10.3916 | 0.00491 |
| $6A''$ | 9.9021 | 0.00350 | $6A''$ | 10.4155 | 0.00304 | $6A''$ | 9.8925 | 0.00327 | $6A''$ | 10.4064 | 0.00277 |
| $7A''$ | 10.0059 | 0.01499 | $5A'$ | 10.4416 | 0.04089 | $7A''$ | 10.0008 | 0.01497 | $5A'$ | 10.4380 | 0.04128 |
| $5A'$ | 10.0267 | 0.04102 | $7A''$ | 10.4536 | 0.01617 | $5A'$ | 10.0212 | 0.04093 | $7A''$ | 10.4512 | 0.01624 |
| $8A''$ | 10.2236 | 0.00728 | $8A''$ | 10.7603 | 0.00835 | $8A''$ | 10.2154 | 0.00719 | $8A''$ | 10.7542 | 0.00799 |
| $6A'$ | 10.3117 | 0.01606 | $6A'$ | 10.8030 | 0.01431 | $6A'$ | 10.3022 | 0.01586 | $6A'$ | 10.7942 | 0.01412 |
| $9A''$ | 10.3459 | 0.00338 | $9A''$ | 10.8052 | 0.00351 | $9A''$ | 10.3354 | 0.00345 | $9A''$ | 10.796 | 0.00383 |
| $7A'$ | 10.8107 | 0.00229 | $7A'$ | 11.2132 | 0.01000 | $7A'$ | 10.8039 | 0.00217 | $7A'$ | 11.2091 | 0.00974 |
| $10A''$ | 10.8845 | 0.00511 | $10A''$ | 11.3563 | 0.00097 | $10A''$ | 10.8805 | 0.00504 | $10A''$ | 11.3536 | 0.00096 |
| $8A'$ | 11.0923 | 0.02914 | $8A'$ | 11.5426 | 0.04864 | $8A'$ | 11.0865 | 0.02887 | $8A'$ | 11.5422 | 0.05151 |
| $9A'$ | 11.2540 | 0.00078 | $9A'$ | 11.5664 | 0.00969 | $9A'$ | 11.2462 | 0.00084 | $9A'$ | 11.5620 | 0.00699 |
| $10A'$ | 11.2963 | 0.03252 | $11A''$ | 11.6661 | 0.05676 | $10A'$ | 11.2985 | 0.03277 | $11A''$ | 11.6638 | 0.05521 |

[a] Mulliken symmetry notation.

Table S8: $CH_3OH$: Unshifted RIXS data at the Oxygen $K$-edge for the pump frequency at resonance with the first core excitation (core $1A'$) calculated using different methods. RIXS cross sections for $\theta = 45^\circ$ at the CVS-uS-EOM-CCSD and CVS-EOM-CCSD level of theory are both based on emission energies calculated at the EOM-CCSD level of theory. CVS and CVS-uS refer to a projection in the damped response solver. All calculations employed the aug-cc-pVTZ basis.

| $\omega_{\text{em}}$/eV | | $\sigma_{45^\circ}^{\text{RIXS}}$/a.u. | | |
|---|---|---|---|---|
| CCSD | CC2 | CVS-uS-EOM-CCSD | CVS-EOM-CCSD | EOM-CC2 |
| 528.5730 | 527.5061 | 0.01759 | 0.01607 | 0.00671 |
| 527.3743 | 526.4288 | 0.00083 | 0.00095 | 0.00012 |
| 526.8636 | 525.9754 | 0.00010 | 0.00013 | 0.00001 |
| 526.7901 | 525.8459 | 0.00003 | 0.00003 | 0.00002 |
| 526.5896 | 525.4704 | 0.01048 | 0.00931 | 0.00437 |
| 526.0796 | 525.1512 | 0.00004 | 0.00017 | 0.00008 |
| 525.7893 | 524.8246 | 0.00038 | 0.00044 | 0.00003 |
| 525.6423 | 524.5601 | 0.00097 | 0.00098 | 0.00014 |
| 525.0970 | 524.1563 | 0.00004 | 0.00009 | 0.00002 |
| 525.0818 | 524.1359 | 0.00036 | 0.00043 | 0.00001 |
| 525.0554 | 524.0322 | 0.00007 | 0.00012 | 0.00000 |
| 525.0434 | 524.0113 | 0.00001 | 0.00004 | 0.00006 |
| 524.7367 | 523.8146 | 0.00022 | 0.00024 | 0.00002 |
| 524.6943 | 523.7264 | 0.00003 | 0.00032 | 0.00001 |
| 524.6918 | 523.6921 | 0.00010 | 0.00020 | 0.00002 |
| 524.2839 | 523.2273 | 0.00130 | 0.00141 | 0.00019 |
| 524.1408 | 523.1536 | 0.00001 | 0.00007 | 0.00000 |
| 523.9544 | 522.9457 | 0.00440 | 0.00398 | 0.00003 |
| 523.9307 | 522.7841 | 0.00135 | 0.00139 | 0.00010 |
| 523.8309 | 522.7419 | 0.00099 | 0.00089 | 0.00215 |

Table S9: $CH_3OH$: Unshifted RIXS data at the Oxygen $K$-edge for the pump frequency at resonance with the second core excitation (core $2A'$) calculated using different methods. RIXS cross sections for $\theta = 45^\circ$ at the CVS-uS-EOM-CCSD and CVS-EOM-CCSD level of theory are both based on emission energies calculated at the EOM-CCSD level of theory. CVS and CVS-uS refer to a projection in the damped response solver. All calculations employed the aug-cc-pVTZ basis.

| $\omega_{em}$/eV | | $\sigma_{45^\circ}^{\text{RIXS}}$/a.u. | | |
|---|---|---|---|---|
| CCSD | CC2 | CVS-uS-EOM-CCSD | CVS-EOM-CCSD | EOM-CC2 |
| 530.6212 | 528.6731 | 0.00053 | 0.00056 | 0.00013 |
| 529.4225 | 527.5958 | 0.00853 | 0.00813 | 0.00192 |
| 528.9118 | 527.1425 | 0.00012 | 0.00012 | 0.00005 |
| 528.8383 | 527.0130 | 0.00058 | 0.00056 | 0.00005 |
| 528.6378 | 526.6375 | 0.00059 | 0.00062 | 0.00012 |
| 528.1278 | 526.3183 | 0.00042 | 0.00060 | 0.00005 |
| 527.8375 | 525.9917 | 0.00019 | 0.00029 | 0.00007 |
| 527.6905 | 525.7272 | 0.00425 | 0.00387 | 0.00102 |
| 527.1452 | 525.3234 | 0.00005 | 0.00011 | 0.00001 |
| 527.1300 | 525.3030 | 0.00010 | 0.00027 | 0.00003 |
| 527.1039 | 525.1993 | 0.00045 | 0.00041 | 0.00003 |
| 527.0919 | 525.1784 | 0.00006 | 0.00005 | 0.00001 |
| 526.7849 | 524.9816 | 0.00004 | 0.00011 | 0.00002 |
| 526.7425 | 524.8935 | 0.00005 | 0.00040 | 0.00001 |
| 526.7403 | 524.8592 | 0.00011 | 0.00024 | 0.00002 |
| 526.3322 | 524.3944 | 0.00015 | 0.00038 | 0.00002 |
| 526.1890 | 524.3207 | 0.00012 | 0.00018 | 0.00000 |
| 526.0026 | 524.1128 | 0.00097 | 0.00097 | 0.00005 |
| 525.9789 | 523.9512 | 0.00005 | 0.00035 | 0.00002 |
| 525.8794 | 523.9087 | 0.00065 | 0.00062 | 0.00016 |

Table S10: $CH_3OH$: Unshifted nonresonant (XES) data at the Oxygen $K$-edge calculated using different methods. All calculations employed the aug-cc-pVTZ basis.

| $\omega_{em}$/eV | | $f_{osc}$ | |
|---|---|---|---|
| CCSD | CC2 | EOM-CCSD | EOM-CC2 |
| 529.4002 | 526.9142 | 0.04350 | 0.04827 |
| 527.5822 | 524.9542 | 0.02846 | 0.03404 |
| 525.1400 | 522.3356 | 0.02045 | 0.01837 |
| 524.5999 | 521.6776 | 0.00911 | 0.00697 |
| 522.6728 | 519.9984 | 0.02611 | 0.02611 |
| 517.2898 | 514.1692 | 0.00556 | 0.00495 |
| 513.7140 | 511.6056 | 0.00001 | 0.00000 |
| 512.9697 | 511.2113 | 0.00000 | 0.00000 |

Table S11: $CH_3OH$: Unshifted RIXS data at the Carbon $K$-edge for the pump frequency at resonance with the first core excitation (core $1A'$) calculated using different methods. RIXS cross sections for $\theta = 45^\circ$ at the CVS-uS-EOM-CCSD and CVS-EOM-CCSD level of theory are both based on emission energies calculated at the EOM-CCSD level of theory. CVS and CVS-uS refer to a projection in the damped response solver. All calculations employed the aug-cc-pVTZ basis.

| $\omega_{em}$/eV | | $\sigma^{\mathrm{RIXS}}_{45^\circ}$/a.u. | | |
|---|---|---|---|---|
| CCSD | CC2 | CVS-uS-EOM-CCSD | CVS-EOM-CCSD | EOM-CC2 |
| 282.1232 | 283.5314 | 0.00495 | 0.00502 | 0.00345 |
| 280.9191 | 282.4503 | 0.00238 | 0.00255 | 0.00135 |
| 280.4089 | 281.9972 | 0.00011 | 0.00032 | 0.00008 |
| 280.3362 | 281.8682 | 0.00007 | 0.00007 | 0.00005 |
| 280.1359 | 281.4935 | 0.01342 | 0.01283 | 0.00942 |
| 279.6276 | 281.1754 | 0.00030 | 0.00055 | 0.00007 |
| 279.3381 | 280.8497 | 0.00003 | 0.00041 | 0.00002 |
| 279.1827 | 280.5784 | 0.00417 | 0.00395 | 0.00265 |
| 278.6442 | 280.1800 | 0.00002 | 0.00021 | 0.00001 |
| 278.6295 | 280.1596 | 0.00006 | 0.00035 | 0.00001 |
| 278.5979 | 280.0510 | 0.00021 | 0.00062 | 0.00034 |
| 278.5846 | 280.0306 | 0.00044 | 0.00071 | 0.0002 |
| 278.2817 | 279.8366 | 0.00054 | 0.00062 | 0.00021 |
| 278.2417 | 279.7498 | 0.00009 | 0.00095 | 0.00003 |
| 278.2398 | 279.7166 | 0.00006 | 0.00042 | 0.00006 |
| 277.8268 | 279.2480 | 0.00477 | 0.00478 | 0.00103 |
| 277.6823 | 279.1713 | 0.00047 | 0.00056 | 0.00005 |
| 277.4937 | 278.9653 | 0.01912 | 0.01798 | 0.00040 |
| 277.4738 | 278.8058 | 0.00383 | 0.00440 | 0.00042 |
| 277.3721 | 278.7536 | 0.01127 | 0.01032 | 0.02205 |

Table S12: $CH_3OH$: Unshifted nonresonant (XES) data at the Carbon $K$-edge calculated using different methods. All calculations employed the aug-cc-pVTZ basis.

| $\omega_{em}$/eV | | $f_{osc}$ | |
|---|---|---|---|
| CCSD | CC2 | EOM-CCSD | EOM-CC2 |
| 282.1594 | 283.0201 | 0.00551 | 0.00416 |
| 280.3381 | 281.0578 | 0.01414 | 0.01194 |
| 277.8888 | 278.4281 | 0.02593 | 0.02828 |
| 277.3448 | 277.7664 | 0.02667 | 0.03002 |
| 275.4262 | 276.0969 | 0.01472 | 0.01677 |
| 270.0133 | 270.2364 | 0.00075 | 0.00129 |
| 266.4646 | 267.7011 | 0.00000 | 0.00000 |

## S2.1 Valence Transition NTOs

| EOM-CCSD | | | EOM-CC2 | | |
|---|---|---|---|---|---|
| Transition Symmetry | Hole NTO | Particle NTO | Transition Symmetry | Hole NTO | Particle NTO |
| 1A'' | 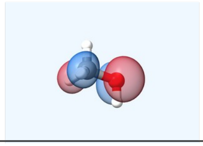 | 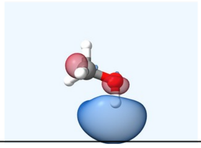 | 1A'' | 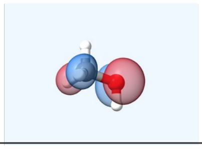 | 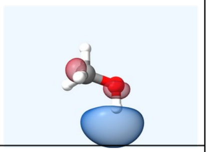 |
| 2A'' | 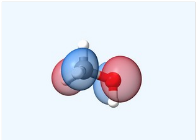 | 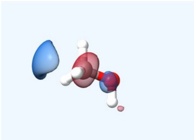 | 2A'' | 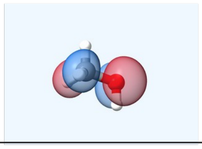 | 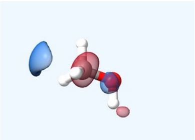 |
| 2A' | 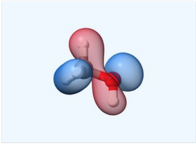 | 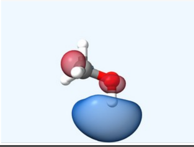 | 2A' | 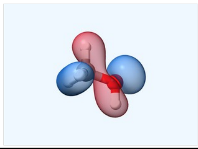 | 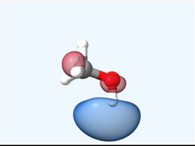 |
| 3A' | 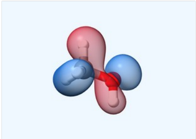 | 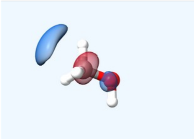 | 3A' | 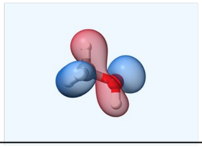 | 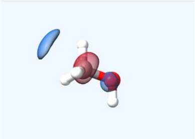 |
| 8A' | 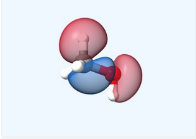 | 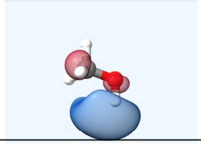 | 10A' | 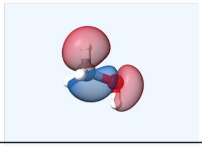 | 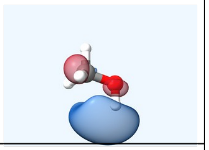 |
| 11A'' | 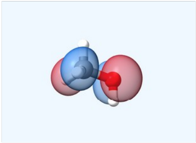 | 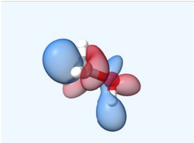 | | | |

Figure S4: $CH_3OH$: NTO pairs of the probed valence transitions at both the CCSD and CC2 levels of theory. Isosurface value was 0.04-0.05 for all NTO pairs.

# S3 $H_2S$

The XAS spectrum for $H_2S$ at the sulfur $K$-edge can be seen in Fig. S5 along with the computed valence absorption spectrum. It can be seen from Fig. S5 that both methods give the same overall shape of the spectrum. Both methods predict a shift between the two first peaks, which is slightly off compared to experiment, but in either direction: While CC2 predicts a too small separation,

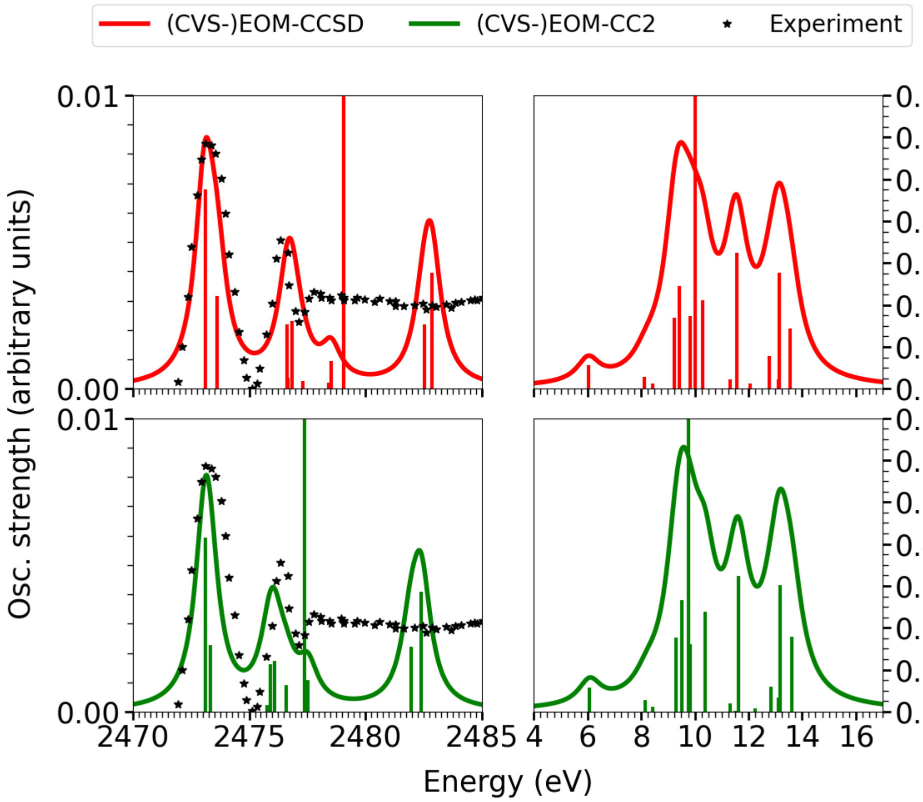


Figure S5: $H_2S$: XAS spectrum at the Sulphur $K$-edge (left) and valence absorption in a space orthogonal to the S core space (right) calculated at the (CVS-)EOM-CC2/6-311++G** (green) and (CVS-)EOM-CCSD/6-311++G** (red) level of theory. Experimental data adapted from Bodeur and Esteva.[2] For all methods 10 core transitions and 20 valence transitions have been determined and plotted. The first core ionization potential is shown as a vertical line spanning the full intensity range. XAS results have been shifted to align with experiment: 3.35 eV for CVS-EOM-CCSD and 4.50 eV for CVS-EOM-CC2. A Lorentzian broadening with HWHM=0.506 eV has been applied.

CCSD predicts one that is too large. The intensity ratio of the first two peaks is slightly better reproduced at the CCSD level of theory. Furthermore, the core ionization threshold appears closer to the two low energy peaks at the CC2 level compared to the CCSD level. Significantly lower CC2 core ionization thresholds compared to CCSD are not uncommon as also observed by Carbone et al.[3] The main transitions of the two peaks below the ionization threshold can in both methods be characterized as core $1B_2$ and core $1B_1$, while the character of the main transition of the small peak (just below the ionization threshold at the CCSD level) is core $3B_2$. Observe that at the CC2 level of theory the third peak falls just above the core ionization threshold.

From the valence spectra in Fig. S5 it is observed that the two methods are in good agreement with each other both regarding the overall spectral profile, the relative intensities of peaks and the position of the ionization threshold relative to the spectral features.

## S3.1 Data tables

Table S13: $H_2S$: Unshifted S $K$-edge XAS data using the 6-311++G** basis set.
[a] Mulliken symmetry notation.

| EOM-CC2 | | | EOM-CCSD | | |
|---|---|---|---|---|---|
| Sym.[a] | $\omega_{abs,c}$/eV | $f_{osc}$ | Sym.[a] | $\omega_{abs,c}$/eV | $f_{osc}$ |
| $1B_2$ | 2468.5932 | 0.00592 | $1B_2$ | 2469.7535 | 0.00678 |
| $1A_1$ | 2468.8162 | 0.00227 | $1A_1$ | 2470.2684 | 0.00317 |
| $2B_2$ | 2471.2486 | 0.00021 | $2A_1$ | 2473.2851 | 0.00219 |
| $2A_1$ | 2471.4052 | 0.00162 | $2B_2$ | 2473.3233 | 0.00038 |
| $1B_1$ | 2471.5780 | 0.00174 | $1B_1$ | 2473.5002 | 0.00231 |
| $3A_1$ | 2472.0885 | 0.00089 | $3A_1$ | 2473.9623 | 0.00027 |
| $3B_2$ | 2473.0127 | 0.00109 | $4A_1$ | 2475.0892 | 0.00022 |
| $4A_1$ | 2473.0275 | 0.00019 | $3B_2$ | 2475.1955 | 0.00094 |
| $4B_2$ | 2477.4436 | 0.00222 | $4B_2$ | 2479.1842 | 0.00218 |
| $5A_1$ | 2477.8977 | 0.00409 | $5A_1$ | 2479.5026 | 0.00397 |

Table S14: $H_2S$: Unshifted valence absorption data computed using the 6-311++G** basis set in a spce orthogonal to the S core space.
[a] Mulliken symmetry notation.

| EOM-CC2 | | | EOM-CCSD | | |
|---|---|---|---|---|---|
| Sym.[a] | $\omega_{abs,v}$/eV | $f_{osc}$ | Sym.[a] | $\omega_{abs,v}$/eV | $f_{osc}$ |
| $1B_1$ | 6.0808 | 0.05768 | $1B_1$ | 6.0274 | 0.05598 |
| $1A_2$ | 6.4085 | 0.00000 | $1A_2$ | 6.3268 | 0.00000 |
| $2A_2$ | 7.8199 | 0.00000 | $2A_2$ | 7.8189 | 0.00000 |
| $2B_1$ | 8.1523 | 0.0282 | $2B_1$ | 8.1334 | 0.02900 |
| $1A_1$ | 8.4299 | 0.01272 | $1A_1$ | 8.4386 | 0.01301 |
| $2A_1$ | 9.2958 | 0.17621 | $2A_1$ | 9.2271 | 0.16897 |
| $3B_1$ | 9.5241 | 0.26584 | $3B_1$ | 9.4191 | 0.24433 |
| $3A_2$ | 9.8380 | 0.00000 | $4B_1$ | 9.8396 | 0.17343 |
| $4B_1$ | 9.8386 | 0.16171 | $3A_2$ | 9.8591 | 0.00000 |
| $1B_2$ | 10.3798 | 0.23896 | $1B_2$ | 10.2891 | 0.21044 |
| $2B_2$ | 10.9891 | 0.00030 | $2B_2$ | 10.9625 | 0.00082 |
| $3A_1$ | 11.3289 | 0.01947 | $3A_1$ | 11.3255 | 0.02220 |
| $5B_1$ | 11.4916 | 0.00111 | $5B_1$ | 11.4787 | 0.00095 |
| $3B_2$ | 11.6126 | 0.32396 | $3B_2$ | 11.5525 | 0.32511 |
| $4A_1$ | 12.2359 | 0.00798 | $4A_1$ | 12.0743 | 0.01220 |
| $5A_1$ | 12.8240 | 0.05979 | $5A_1$ | 12.7794 | 0.07902 |
| $4B_2$ | 13.1295 | 0.03343 | $4B_2$ | 13.1249 | 0.02242 |
| $6A_1$ | 13.1775 | 0.30105 | $6A_1$ | 13.143 | 0.27669 |
| $7A_1$ | 13.6175 | 0.17971 | $7A_1$ | 13.5465 | 0.14309 |
| $5B_2$ | 13.8736 | 0.00060 | $5B_2$ | 13.7782 | 0.00018 |

Table S15: $H_2S$: Unshifted RIXS data for the pump frequency at resonance with the first core excitation (core $1B_2$ in Mulliken symmetry notation) calculated using different methods. RIXS cross sections for $\theta = 45^\circ$ at the EOM-CCSD, CVS-uS-EOM-CCSD and CVS-EOM-CCSD level of theory are all based on emission energies calculated at the EOM-CCSD level of theory. CVS and CVS-uS refer to a projection in the damped response solver. To avoid reporting very small numbers all calculated cross sections have been multiplied with $10^3$. All calculations employed the 6-311++G** basis.

| $\omega_{em}$/eV | | $10^3\sigma^{\mathrm{RIXS}}_{45^\circ}$/a.u. | | | |
|---|---|---|---|---|---|
| CCSD | CC2 | EOM-CCSD | CVS-uS-EOM-CCSD | CVS-EOM-CCSD | EOM-CC2 |
| 2463.7261 | 2462.5125 | 0.00084 | 0.00101 | 0.00114 | 0.00333 |
| 2463.4265 | 2462.1849 | 0.08424 | 0.10229 | 0.07107 | 0.07717 |
| 2461.9345 | 2460.7734 | 0.05791 | 0.05480 | 0.01905 | 0.05859 |
| 2461.6200 | 2460.4409 | 0.05539 | 0.05384 | 0.02322 | 0.05715 |
| 2461.3149 | 2460.1634 | 0.00031 | 0.00047 | 0.15542 | 0.00027 |
| 2460.5264 | 2459.2975 | 0.00096 | 0.00073 | 0.00824 | 0.00220 |
| 2460.3345 | 2459.0692 | 0.06058 | 0.05535 | 0.01417 | 0.06378 |
| 2459.9138 | 2458.7552 | 0.04814 | 0.04638 | 0.01607 | 0.05045 |
| 2459.8942 | 2458.7546 | 0.05204 | 0.04727 | 0.02233 | 0.04415 |
| 2459.4643 | 2458.2134 | 0.03201 | 0.03769 | 0.04086 | 0.02874 |
| 2458.7911 | 2457.6041 | 0.02460 | 0.02462 | 0.05278 | 0.02466 |
| 2458.4281 | 2457.2643 | 0.00086 | 0.00097 | 0.0306 | 0.000550 |
| 2458.2749 | 2457.1015 | 0.02357 | 0.02346 | 0.00959 | 0.02375 |
| 2458.2009 | 2456.9807 | 0.01069 | 0.01153 | 0.00461 | 0.01327 |
| 2457.6792 | 2456.3573 | 0.00837 | 0.00909 | 0.00936 | 0.00730 |
| 2456.9742 | 2455.7693 | 0.00582 | 0.00632 | 0.01429 | 0.00553 |
| 2456.6286 | 2455.4637 | 0.00337 | 0.00369 | 0.00422 | 0.00244 |
| 2456.6104 | 2455.4158 | 0.00490 | 0.00535 | 0.01194 | 0.00516 |
| 2456.2068 | 2454.9758 | 0.00204 | 0.00228 | 0.01636 | 0.00261 |
| 2455.9752 | 2454.7197 | 0.01208 | 0.01194 | 0.02731 | 0.01196 |

Table S16: $H_2S$: Unshifted RIXS data for the pump frequency at resonance with the second core excitation (core $1A_1$ in Mulliken symmetry notation) calculated using different methods. RIXS cross sections for $\theta = 45^\circ$ at the EOM-CCSD, CVS-uS-EOM-CCSD and CVS-EOM-CCSD level of theory are all based on emission energies calculated at the EOM-CCSD level of theory. CVS and CVS-uS refer to a projection in the damped response solver. To avoid reporting very small numbers all calculated cross sections have been multiplied with $10^3$. All calculations employed the 6-311++G** basis.

| $\omega_{em}$/eV | | $10^3\sigma^{\mathrm{RIXS}}_{45^\circ}$/a.u. | | | |
|---|---|---|---|---|---|
| CCSD | CC2 | EOM-CCSD | CVS-uS-EOM-CCSD | CVS-EOM-CCSD | EOM-CC2 |
| 2464.2410 | 2462.7354 | 0.02312 | 0.02574 | 0.02506 | 0.00002 |
| 2463.9417 | 2462.4078 | 0.07451 | 0.06620 | 0.02917 | 0.06808 |
| 2462.4494 | 2460.9963 | 0.05521 | 0.05340 | 0.01804 | 0.05588 |
| 2462.1351 | 2460.6638 | 0.05598 | 0.05329 | 0.02269 | 0.05585 |
| 2461.8298 | 2460.3862 | 0.00067 | 0.00083 | 0.15507 | 0.00000 |
| 2461.0412 | 2459.5203 | 0.01319 | 0.01452 | 0.01941 | 0.00002 |
| 2460.8494 | 2459.2920 | 0.06173 | 0.06113 | 0.01894 | 0.06683 |
| 2460.4289 | 2458.9780 | 0.04912 | 0.04546 | 0.01536 | 0.04397 |
| 2460.4093 | 2458.9775 | 0.04290 | 0.04166 | 0.01748 | 0.04285 |
| 2459.9794 | 2458.4365 | 0.00732 | 0.00753 | 0.00625 | 0.00314 |
| 2459.3059 | 2457.8273 | 0.02739 | 0.02926 | 0.05412 | 0.02889 |
| 2458.9429 | 2457.4871 | 0.00026 | 0.00027 | 0.03016 | 0.00000 |
| 2458.7897 | 2457.3247 | 0.02369 | 0.02367 | 0.00970 | 0.02323 |
| 2458.7160 | 2457.2036 | 0.02363 | 0.02123 | 0.01479 | 0.00934 |
| 2458.1941 | 2456.5802 | 0.00122 | 0.00125 | 0.00151 | -0.00001 |
| 2457.4890 | 2455.9921 | 0.00042 | 0.00045 | 0.00562 | 0.00000 |
| 2457.1434 | 2455.6868 | 0.00022 | 0.00015 | 0.00038 | 0.00003 |
| 2457.1255 | 2455.6386 | 0.00093 | 0.00095 | 0.00500 | 0.00000 |
| 2456.7219 | 2455.1986 | 0.00034 | 0.00044 | 0.01692 | 0.00000 |
| 2456.4901 | 2454.9426 | 0.01247 | 0.01205 | 0.02713 | 0.01184 |

Table S17: $H_2S$: Unshifted RIXS data for the pump frequency at resonance with the 3rd (CCSD) or 4th (CC2) core excitation (core $2A_1$ in Mulliken symmetry notation) calculated using different methods. RIXS cross sections for $\theta = 45^\circ$ at the EOM-CCSD, CVS-uS-EOM-CCSD and CVS-EOM-CCSD level of theory are all based on emission energies calculated at the EOM-CCSD level of theory. CVS and CVS-uS refer to a projection in the damped response solver. To avoid reporting very small numbers all calculated cross sections have been multiplied with $10^3$. All calculations employed the 6-311++G** basis.

| $\omega_{em}$/eV | | $10^3\sigma_{45^\circ}^{\mathrm{RIXS}}$/a.u. | | | |
|---|---|---|---|---|---|
| CCSD | CC2 | EOM-CCSD | CVS-uS-EOM-CCSD | CVS-EOM-CCSD | EOM-CC2 |
| 2467.2576 | 2465.3243 | 0.00114 | 0.00097 | 0.00091 | 0.00035 |
| 2466.9583 | 2464.9966 | 0.05508 | 0.04866 | 0.01655 | 0.05445 |
| 2465.4663 | 2463.5852 | 0.06610 | 0.06196 | 0.02542 | 0.04952 |
| 2465.1517 | 2463.2529 | 0.07656 | 0.06614 | 0.03595 | 0.07570 |
| 2464.8464 | 2462.9754 | 0.00314 | 0.00485 | 0.19695 | 0.00318 |
| 2464.0581 | 2462.1095 | 0.00096 | 0.00116 | 0.00732 | 0.00042 |
| 2463.8660 | 2461.8812 | 0.06221 | 0.06141 | 0.01891 | 0.06400 |
| 2463.4456 | 2461.5672 | 0.04756 | 0.04549 | 0.01520 | 0.04740 |
| 2463.4260 | 2461.5666 | 0.04715 | 0.04562 | 0.02102 | 0.04442 |
| 2462.9961 | 2461.0254 | 0.00235 | 0.00230 | 0.00664 | 0.00210 |
| 2462.3226 | 2460.4161 | 0.03441 | 0.03220 | 0.05743 | 0.02589 |
| 2461.9596 | 2460.0763 | 0.00709 | 0.00794 | 0.03529 | 0.00616 |
| 2461.8064 | 2459.9136 | 0.03676 | 0.03790 | 0.02228 | 0.03652 |
| 2461.7326 | 2459.7925 | 0.00728 | 0.00742 | 0.00211 | 0.00569 |
| 2461.2110 | 2459.1693 | 0.00105 | 0.00110 | 0.00156 | 0.00045 |
| 2460.5057 | 2458.5813 | 0.00036 | 0.00042 | 0.00831 | 0.00017 |
| 2460.1604 | 2458.2757 | 0.00015 | 0.00019 | 0.00078 | 0.00006 |
| 2460.1421 | 2458.2278 | 0.00053 | 0.00059 | 0.00723 | 0.00046 |
| 2459.7386 | 2457.7878 | 0.00134 | 0.00169 | 0.01829 | 0.00039 |
| 2459.5070 | 2457.5315 | 0.02493 | 0.02167 | 0.03582 | 0.02284 |

Table S18: $H_2S$: Unshifted RIXS data for the pump frequency at resonance with the fifth core excitation (core $1B_1$ in Mulliken symmetry notation) calculated using different methods. RIXS cross sections for $\theta = 45^{\circ}$ at the EOM-CCSD, CVS-uS-EOM-CCSD and CVS-EOM-CCSD level of theory are all based on emission energies calculated at the EOM-CCSD level of theory. CVS and CVS-uS refer to a projection in the damped response solver. To avoid reporting very small numbers all calculated cross sections have been multiplied with $10^3$. All calculations employed the 6-311++G** basis.

| $\omega_{em}$/eV | | $10^3\sigma_{45^{\circ}}^{\text{RIXS}}$/a.u. | | | |
|---|---|---|---|---|---|
| CCSD | CC2 | EOM-CCSD | CVS-uS-EOM-CCSD | CVS-EOM-CCSD | EOM-CC2 |
| 2467.4729 | 2465.4971 | 0.00011 | 0.00006 | 0.00006 | 0.00007 |
| 2467.1733 | 2465.1694 | 0.05364 | 0.04752 | 0.01575 | 0.05442 |
| 2465.6813 | 2463.7580 | 0.04678 | 0.04513 | 0.01194 | 0.05098 |
| 2465.3667 | 2463.4257 | 0.03663 | 0.03532 | 0.00810 | 0.03935 |
| 2465.0617 | 2463.1482 | 0.01483 | 0.01623 | 0.16618 | 0.01131 |
| 2464.2731 | 2462.2823 | 0.00056 | 0.00055 | 0.00640 | 0.00040 |
| 2464.0810 | 2462.0540 | 0.07194 | 0.06489 | 0.02044 | 0.06844 |
| 2463.6606 | 2461.7400 | 0.04666 | 0.04462 | 0.01483 | 0.04772 |
| 2463.6410 | 2461.7394 | 0.04648 | 0.04511 | 0.02057 | 0.04332 |
| 2463.2110 | 2461.1982 | 0.00286 | 0.00275 | 0.00631 | 0.00191 |
| 2462.5378 | 2460.5889 | 0.02268 | 0.02177 | 0.04182 | 0.02654 |
| 2462.1748 | 2460.2491 | 0.00296 | 0.00225 | 0.01772 | 0.00365 |
| 2462.0216 | 2460.0863 | 0.04223 | 0.03702 | 0.02346 | 0.03894 |
| 2461.9476 | 2459.9653 | 0.00673 | 0.00659 | 0.00155 | 0.00594 |
| 2461.4260 | 2459.3421 | 0.00029 | 0.00043 | 0.00066 | 0.00016 |
| 2460.7206 | 2458.7541 | 0.00020 | 0.00019 | 0.00697 | 0.00011 |
| 2460.3753 | 2458.4485 | 0.00005 | 0.00004 | 0.00087 | 0.00003 |
| 2460.3571 | 2458.4006 | 0.00025 | 0.00023 | 0.00461 | 0.00015 |
| 2459.9536 | 2457.9606 | 0.00060 | 0.00035 | 0.01200 | 0.00008 |
| 2459.7220 | 2457.7043 | 0.00706 | 0.00647 | 0.01522 | 0.00790 |

Table S19: $H_2S$: Unshifted RIXS data for the pump frequency at resonance with the 8th (EOM-CCSD) and 7th (EOM-CC2) core excitation (core $3B_2$ in Mulliken symmetry notation). RIXS cross sections for $\theta = 45°$ at the EOM-CCSD, CVS-uS-EOM-CCSD and CVS-EOM-CCSD level of theory are all based on emission energies calculated at the EOM-CCSD level of theory. CVS and CVS-uS refer to a projection in the damped response solver. To avoid reporting very small numbers all calculated cross sections have been multiplied with $10^3$. All calculations employed the 6-311++G** basis.

| $\omega_{em}$/eV | | $10^3\sigma_{45°}^{\mathrm{RIXS}}$/a.u. | | | |
|---|---|---|---|---|---|
| CCSD | CC2 | EOM-CCSD | CVS-uS-EOM-CCSD | CVS-EOM-CCSD | EOM-CC2 |
| 2469.1682 | 2466.9319 | 0.00005 | 0.00001 | 0.00002 | 0.00001 |
| 2468.8686 | 2466.6043 | 0.05485 | 0.04721 | 0.01562 | 0.05479 |
| 2467.3766 | 2465.1928 | 0.05352 | 0.05217 | 0.01716 | 0.05489 |
| 2467.0620 | 2464.8603 | 0.05065 | 0.04901 | 0.01909 | 0.05232 |
| 2466.7569 | 2464.5828 | 0.00011 | 0.00001 | 0.14283 | 0.00011 |
| 2465.9684 | 2463.7169 | 0.00003 | 0.00003 | 0.00560 | 0.00001 |
| 2465.7765 | 2463.4886 | 0.06749 | 0.06192 | 0.01844 | 0.07600 |
| 2465.3558 | 2463.1746 | 0.04067 | 0.03797 | 0.01016 | 0.06226 |
| 2465.3362 | 2463.1740 | 0.05946 | 0.05204 | 0.02731 | 0.04612 |
| 2464.9063 | 2462.6328 | 0.00350 | 0.00291 | 0.00743 | 0.00255 |
| 2464.2331 | 2462.0235 | 0.02612 | 0.02528 | 0.04890 | 0.02878 |
| 2463.8701 | 2461.6837 | 0.00002 | 0.00001 | 0.02669 | 0.00003 |
| 2463.7169 | 2461.5209 | 0.02062 | 0.02052 | 0.00715 | 0.02040 |
| 2463.6429 | 2461.4001 | 0.00795 | 0.00758 | 0.00207 | 0.00730 |
| 2463.1212 | 2460.7767 | 0.00015 | 0.00030 | 0.00057 | 0.00027 |
| 2462.4162 | 2460.1887 | 0.00084 | 0.00072 | 0.00900 | 0.00087 |
| 2462.0706 | 2459.8831 | 0.00487 | 0.00539 | 0.00582 | 0.00571 |
| 2462.0526 | 2459.8352 | 0.00069 | 0.00065 | 0.00582 | 0.00048 |
| 2461.6491 | 2459.3952 | 0.00005 | 0.00007 | 0.01446 | 0.00009 |
| 2461.4173 | 2459.1391 | 0.01065 | 0.01045 | 0.02455 | 0.01054 |

Table S20: $H_2S$: Unshifted nonresonant (XES) data at the sulfur $K$-edge calculated using different methods. All calculations employed the 6-311++G** basis.

| $\omega_{em}$/eV | | $f_{osc}$ | |
|---|---|---|---|
| CCSD | CC2 | EOM-CCSD | EOM-CC2 |
| 2465.7156 | 2463.1172 | 0.00606 | 0.00596 |
| 2462.5702 | 2459.9897 | 0.00431 | 0.00423 |
| 2460.1299 | 2457.4858 | 0.00378 | 0.00368 |
| 2454.1529 | 2450.8764 | 0.00001 | 0.00000 |
| 2453.3847 | 2449.2957 | 0.00013 | 0.00002 |
| 2452.6459 | 2449.0717 | 0.00000 | 0.00022 |
| 2451.5814 | 2449.0551 | 0.00012 | 0.00001 |

## S3.2 Valence Transition NTOs

| EOM-CCSD | | | EOM-CC2 | | |
|---|---|---|---|---|---|
| Transition Symmetry | Hole NTO | Particle NTO | Transition Symmetry | Hole NTO | Particle NTO |
| $1A_2$ | 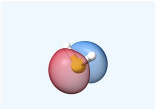 | 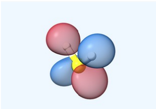 | $1A_2$ | 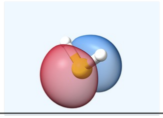 | 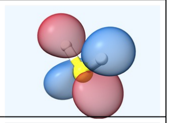 |
| $2A_2$ | 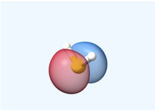 | 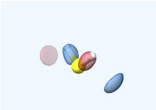 | $2A_2$ | 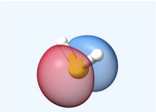 | 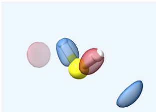 |
| $2B_1$ | 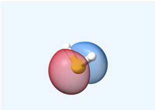 | 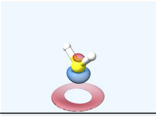 | $2B_1$ | 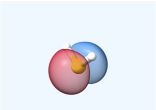 | 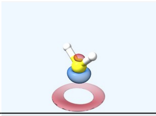 |
| $1A_1$ | 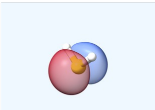 | 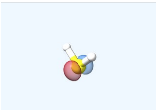 | | | |
| $3B_1$ | 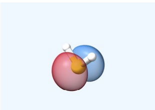 | 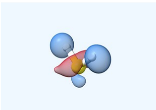 | $3B_1$ | 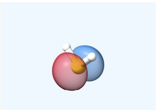 | 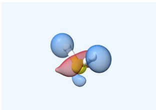 |
| $4B_1$ | 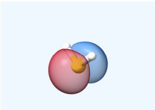 | 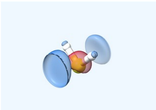 | $4B_1$ | 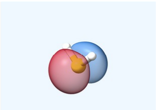 | 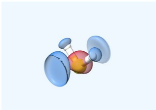 |
| $3A_2$ | 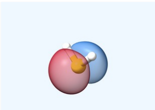 | 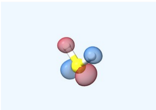 | $3A_2$ | 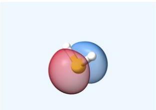 | 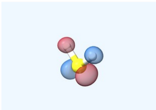 |
| $2B_2$ | 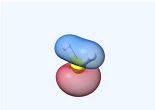 | 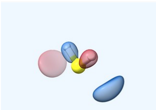 | | | |
| $5B_1$ | 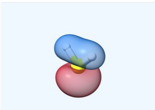 | 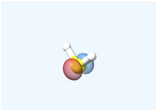 | $5B_1$ | 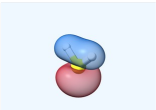 | 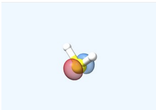 |

Figure S6: $H_2S$: NTO pairs of the probed valence transitions at both the CCSD and CC2 levels of theory. Isosurface value was 0.04-0.06 for all NTO pairs.

# S4 Para-nitro-aniline

The XAS spectrum is computed at both the CVS-EOM-CCSD and the CVS-EOM-CC2 level of theory at the C *K*-edge (see Fig. S7). We observe that the core transitions are significantly more close-lying, according to the CVS-EOM-CC2 calculation compared to the CVS-EOM-CCSD one. The latter is in better agreement with experiment. The intensity ratios of the first three bright

transitions predicted are however very similar in the two methods, and they both find the first bright transition to be core $1B_1$. We note that the EOM-CC2 and EOM-CCSD valence spectra in

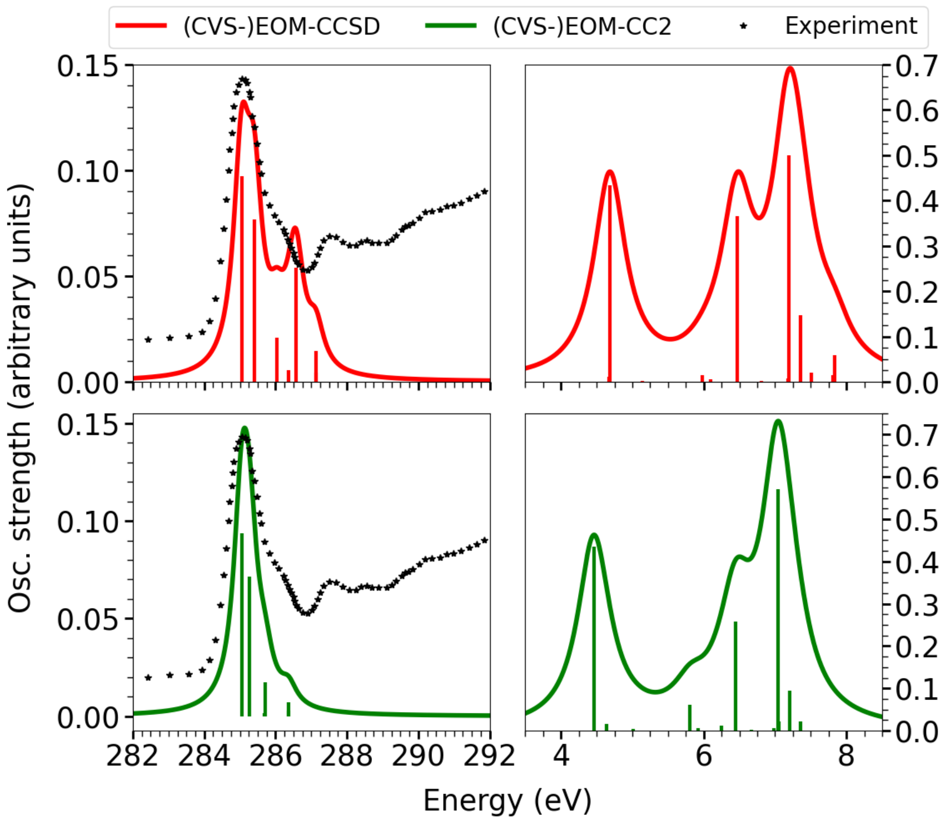


Figure S7: PNA: XAS spectra at the Carbon $K$-edge (left) and valence absorption (right) in the space orthogonal to the C core space, calculated using (CVS-)EOM-CC2/6-311++G** (green) and (CVS-)EOM-CCSD/6-311++G** (red) levels of theory. For all methods, 10 core transitions and 20 valence transitions were computed. A Lorentzian broadening with HWHM=0.27 eV has been applied. The theoretical spectra were shifted by $-1.70$ eV (CVS-EOM-CCSD) and $-2.94$ eV (CVS-EOM-CC2) to align with experiment, which was digitized from Turci et al.[4]

Fig. S7 are very similar. The general shape is the same, however the shift between the first and second feature is larger when using EOM-CC2. The low intensity feature between the two main peaks at low energy is also more pronounced when employing EOM-CC2.

## S4.1 Comparison of CVS-EOM-CCSD, CVS-0-EOM-CCSD and fc-CVS-0-EOM-CCSD

We investigate here whether the discrepancies between the calculated CVS-EOM-CCSD and fc-CVS-0-EOM-CCSD RIXS results are mainly due to the fc approximation or to the way our projectors are applied. Both CVS approximations consist in projecting out all excitations that do not involve a core orbital when solving the damped response equations. While this is done for all damped response equations for CVS-0, it is only done for the divergent damped response equations for CVS.

Therefore, we calculate, for a small basis set (6-31G), the RIXS spectra using the different projection schemes. The results are then compared to the fc-CVS-0-EOM-CCSD result calculated with Q-Chem (see Fig. S8). Here, it is noted that the CVS-0-EOM-CCSD and fc-CVS-0-EOM-CCSD are almost identical, with only a small overall decrease in intensity of the fc-CVS-0-EOM-CCSD result compared to CVS-0-EOM-CCSD. The CVS-EOM-CCSD result, on the other hand, shows larger discrepancies with these other spectra with respect to intensities, while it is still the same transitions that are probed. We thus conclude that the discrepancies are a result of the different ways the projection is applied, rather than an effect of the frozen core approximation.

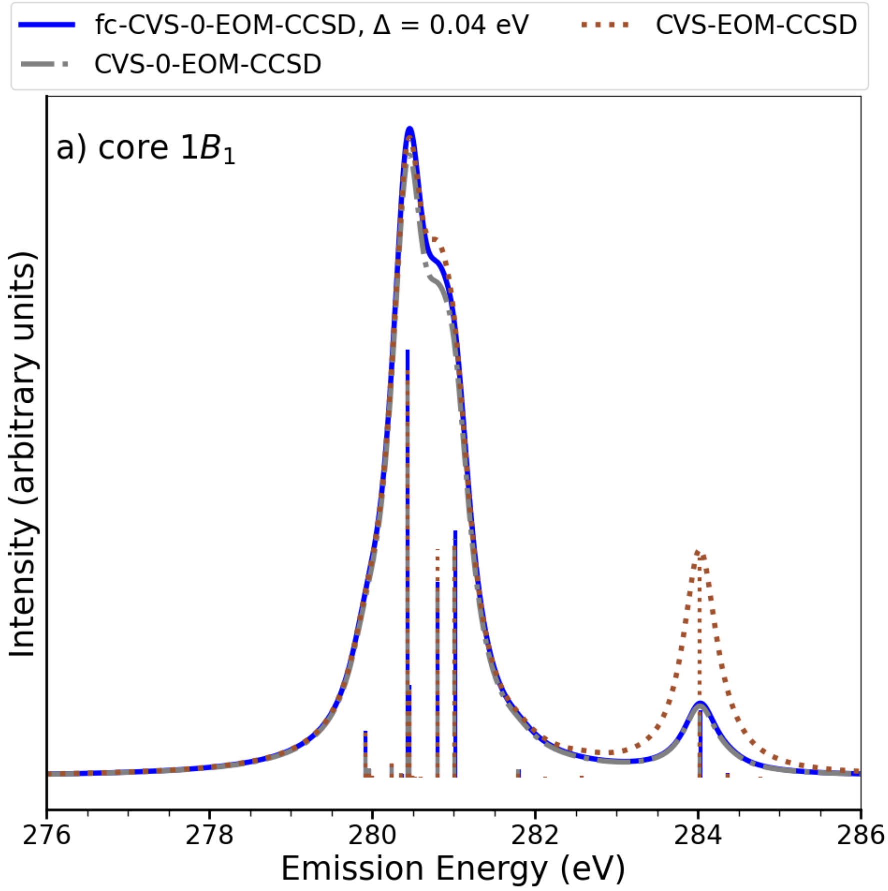


Figure S8: PNA: Comparison of the RIXS spectra at resonance with the energy of the first core excitation at the C *K*-edge (288.90 eV at the CVS-EOM-CCSD level of theory in $e^T$ and 288.86 eV at the fc-CVS-0-EOM-CCSD level of theory in Q-Chem). The results are obtained using different CVS schemes during the solution of the damped response equations. The 6-31G basis set was employed in all calculations. The results are shifted based on the CVS-EOM-CCSD RIXS results. A Lorentzian broadening was applied with HWHM=0.27 eV.

## S4.2 Data tables

Table S21: PNA: Unshifted C $K$-edge XAS data using the 6-311++G** basis set.
[a] Mulliken symmetry notation.

| EOM-CC2 | | | EOM-CCSD | | |
|---|---|---|---|---|---|
| Sym.[a] | $\omega_{abs,c}$/eV | $f_{osc}$ | Sym.[a] | $\omega_{abs,c}$/eV | $f_{osc}$ |
| $1A_2$ | 287.9911 | 0.00000 | $1A_2$ | 286.7436 | 0.00000 |
| $1B_1$ | 287.9948 | 0.09372 | $1B_1$ | 286.7476 | 0.09708 |
| $2A_2$ | 288.2064 | 0.00000 | $2A_2$ | 287.0951 | 0.00000 |
| $2B_1$ | 288.2094 | 0.07154 | $2B_1$ | 287.0984 | 0.07664 |
| $3B_1$ | 288.6269 | 0.00145 | $3B_1$ | 287.7333 | 0.02084 |
| $3A_2$ | 288.6278 | 0.00000 | $4B_1$ | 288.0689 | 0.00555 |
| $4B_1$ | 288.6511 | 0.01726 | $3A_2$ | 288.0712 | 0.00000 |
| $1B_2$ | 289.3100 | 0.00716 | $5B_1$ | 288.2635 | 0.05398 |
| $1A_1$ | 289.3102 | 0.00273 | $1B_1$ | 288.8292 | 0.01455 |
| $4A_2$ | 289.3468 | 0.00000 | $1A_1$ | 288.8302 | 0.00443 |

Table S22: PNA: Unshifted valence absorption data computed using the 6-311++G** basis set in a space orthogonal to the C core space.

| EOM-CC2 | | | EOM-CCSD | | |
|---|---|---|---|---|---|
| Sym.[a] | $\omega_{abs,v}$/eV | $f_{osc}$ | Sym.[a] | $\omega_{abs,v}$/eV | $f_{osc}$ |
| $1A_2$ | 4.0521 | 0.00000 | $1A_2$ | 4.1467 | 0.00000 |
| $1A_1$ | 4.4589 | 0.43494 | $1B_2$ | 4.6753 | 0.01140 |
| $1B_2$ | 4.6369 | 0.01648 | $1B_1$ | 4.6841 | 0.00051 |
| $1B_1$ | 4.6579 | 0.00057 | $1A_1$ | 4.6844 | 0.43385 |
| $2B_1$ | 5.0109 | 0.00298 | $2B_1$ | 5.1392 | 0.00250 |
| $2A_2$ | 5.7592 | 0.00000 | $2A_2$ | 5.9266 | 0.00000 |
| $2B_2$ | 5.8044 | 0.06039 | $2B_2$ | 5.9810 | 0.01432 |
| $3B_1$ | 5.9175 | 0.00576 | $3B_1$ | 6.0947 | 0.00633 |
| $2A_1$ | 6.2502 | 0.01174 | $2A_1$ | 6.4433 | -0.00002 |
| $3B_2$ | 6.4481 | 0.25818 | $3B_2$ | 6.4703 | 0.36542 |
| $4B_1$ | 6.6715 | 0.00262 | $4B_1$ | 6.8102 | 0.00231 |
| $3A_2$ | 6.6750 | 0.00000 | $3A_2$ | 6.8696 | 0.00000 |
| $5B_1$ | 6.7867 | 0.00014 | $4A_2$ | 6.9744 | 0.00000 |
| $4A_2$ | 6.8330 | 0.00000 | $5B_1$ | 7.1809 | 0.00778 |
| $6B_1$ | 6.9840 | 0.00588 | $3A_1$ | 7.1893 | 0.49992 |
| $3A_1$ | 7.0363 | 0.57029 | $4A_1$ | 7.3523 | 0.14729 |
| $4B_2$ | 7.0557 | 0.02146 | $6B_1$ | 7.5075 | 0.02095 |
| $5A_2$ | 7.1435 | 0.00000 | $5A_2$ | 7.6409 | 0.00000 |
| $4A_1$ | 7.2035 | 0.09528 | $5A_1$ | 7.8131 | 0.01506 |
| $7B_1$ | 7.3555 | 0.02174 | $4B_2$ | 7.8375 | 0.05817 |

[a] Mulliken symmetry notation.

Table S23: PNA: Unshifted RIXS data for the pump frequency at resonance with the first bright core excitation (core $1B_1$ in Mulliken symmetry notation) calculated using different methods. RIXS cross sections for $\theta = 45^\circ$ at the CVS-uS-EOM-CCSD and CVS-EOM-CCSD level of theory are both based on emission energies calculated at the EOM-CCSD level of theory. CVS and CVS-uS refer to different types of projections in the damped response solver. All calculations employed the 6-311++G** basis.

| $\omega_{em}$/eV | | | $\sigma^{\mathrm{RIXS}}_{45^\circ}$/a.u. | | | |
|---|---|---|---|---|---|---|
| CCSD | fc-CCSD | CC2 | CVS-uS-EOM-CCSD | CVS-EOM-CCSD | fc-CVS-0-EOM-CCSD | EOM-CC2 |
| 282.6010 | 282.0870 | 283.9428 | 0.00001 | 0.00001 | 0.00000 | 0.00001 |
| 282.0723 | 281.5863 | 283.5360 | 0.00006 | 0.00002 | 0.00000 | 0.01769 |
| 282.0636 | 281.5672 | 283.3580 | 0.00153 | 0.00114 | 0.02000 | 0.00010 |
| 282.0633 | 281.5509 | 283.3371 | 0.02315 | 0.04831 | 0.00000 | 0.00244 |
| 281.6083 | 281.1101 | 282.9839 | 0.00001 | 0.00047 | 0.00000 | 0.00002 |
| 280.8208 | 280.3210 | 282.2356 | 0.00004 | 0.00011 | 0.00000 | 0.00003 |
| 280.7667 | 280.2693 | 282.1904 | 0.00036 | 0.00033 | 0.00000 | 0.00023 |
| 280.6529 | 280.1577 | 282.0775 | 0.00003 | 0.00032 | 0.00000 | 0.00002 |
| 280.3044 | 279.8094 | 281.7447 | 0.00232 | 0.00536 | 0.00000 | 0.00234 |
| 280.2774 | 279.7740 | 281.5468 | 0.00004 | -0.00001 | 0.00000 | 0.00000 |
| 279.9375 | 279.4420 | 281.3234 | 0.00012 | 0.00013 | 0.00000 | 0.00011 |
| 279.8780 | 279.3794 | 281.3199 | 0.00008 | 0.00028 | 0.00000 | 0.00008 |
| 279.7732 | 279.2815 | 281.2080 | 0.00005 | 0.00182 | 0.00000 | 0.02206 |
| 279.5667 | 279.0720 | 281.1618 | 0.00005 | 0.00016 | 0.07000 | 0.00008 |
| 279.5582 | 279.0692 | 281.0108 | 0.07177 | 0.06147 | 0.00000 | 0.00003 |
| 279.3952 | 278.9005 | 280.9585 | 0.00769 | 0.00653 | 0.01000 | 0.04890 |
| 279.2401 | 278.7454 | 280.9392 | 0.00001 | 0.00006 | 0.00000 | 0.00000 |
| 279.1068 | 278.6148 | 280.8513 | 0.00007 | 0.00050 | 0.00000 | 0.01321 |
| 278.9345 | 278.4407 | 280.7914 | 0.04520 | 0.05061 | 0.04000 | 0.01238 |
| 278.9100 | 278.4162 | 280.6393 | 0.00003 | 0.00031 | 0.00000 | 0.00000 |

Table S24: PNA: Unshifted nonresonant (XES) data at the Carbon $K$-edge for C1-C3 (the numbering is based on energies, so that first core excitation from 1s(C1) has the lowest energy), calculated using different methods. All calculations employed the 6-311++G** basis.

| C1 | | | | C2 | | | | C3 | | | |
|---|---|---|---|---|---|---|---|---|---|---|---|
| EOM-CCSD | | EOM-CC2 | | EOM-CCSD | | EOM-CC2 | | EOM-CCSD | | EOM-CC2 | |
| $\omega_{em}$/eV | $f_{osc}$ | $\omega_{em}$/eV | $f_{osc}$ | $\omega_{em}$/eV | $f_{osc}$ | $\omega_{em}$/eV | $f_{osc}$ | $\omega_{em}$/eV | $f_{osc}$ | $\omega_{em}$/eV | $f_{osc}$ |
| 283.9697 | 0.01763 | 283.7159 | 0.01693 | 283.9703 | 0.00000 | 283.7164 | 0.00000 | 284.4005 | 0.00070 | 284.2791 | 0.00001 |
| 282.4720 | 0.00000 | 282.6554 | 0.00000 | 282.4726 | 0.02606 | 282.6560 | 0.00052 | 282.9028 | 0.00000 | 283.2187 | 0.00002 |
| 281.7985 | 0.00000 | 282.2347 | 0.00051 | 281.7991 | 0.00064 | 282.2353 | 0.00006 | 282.2293 | 0.00000 | 282.7980 | 0.00135 |
| 281.4744 | 0.00000 | 282.1681 | 0.00000 | 281.4750 | 0.00041 | 282.1686 | 0.02680 | 281.9049 | 0.00000 | 282.7311 | 0.00000 |
| 281.4255 | 0.00078 | 281.3572 | 0.00000 | 281.426 | 0.00009 | 281.3577 | 0.00080 | 281.8560 | 0.00082 | 281.9204 | 0.00000 |
| 280.6467 | 0.00076 | 280.6829 | 0.00059 | 280.6472 | 0.00000 | 280.6834 | 0.00000 | 281.0772 | 0.01227 | 281.2461 | 0.00837 |
| 279.5800 | 0.01806 | 279.7433 | 0.01825 | 279.5805 | 0.00020 | 279.7438 | 0.00030 | 280.0105 | 0.01615 | 280.3063 | 0.02084 |
| 278.6028 | 0.01063 | 278.7171 | 0.01240 | 278.6034 | 0.00000 | 278.7177 | 0.00000 | 279.0336 | 0.00620 | 279.2801 | 0.00507 |
| 278.1438 | 0.02309 | 278.4390 | 0.02361 | 278.1443 | 0.00016 | 278.4396 | 0.00019 | 278.5745 | 0.02122 | 279.0023 | 0.02287 |
| 277.3277 | 0.00947 | 277.6213 | 0.00602 | 277.3282 | 0.01293 | 277.6219 | 0.01362 | 277.7585 | 0.01103 | 278.1846 | 0.01289 |
| 277.1742 | 0.00615 | 277.4768 | 0.01060 | 277.1748 | 0.01284 | 277.4774 | 0.01295 | 277.6047 | 0.01059 | 278.0401 | 0.01186 |
| 276.6376 | 0.00238 | 276.7848 | 0.00197 | 276.6382 | 0.01386 | 276.7854 | 0.01461 | 277.0684 | 0.00000 | 277.3481 | 0.00011 |
| 275.4488 | 0.00002 | 276.2199 | 0.00011 | 275.4493 | 0.00068 | 276.2205 | 0.00101 | 275.8792 | 0.00098 | 276.7829 | 0.00253 |
| 275.3328 | 0.00002 | 275.4983 | 0.00001 | 275.3334 | 0.00000 | 275.4988 | 0.00000 | 275.7636 | 0.00035 | 276.0613 | 0.00015 |
| 274.6996 | 0.00022 | 275.4011 | 0.00117 | 274.7002 | 0.00117 | 275.4017 | 0.00000 | 275.1301 | 0.00124 | 275.9644 | 0.00051 |
| 274.5037 | -0.00002 | 274.5040 | 0.00089 | 274.5042 | 0.00000 | 274.5045 | 0.00496 | 274.9342 | 0.00004 | 275.0670 | 0.00180 |
| 274.1717 | 0.00082 | 274.4509 | 0.00086 | 274.1723 | 0.00094 | 274.4515 | 0.00063 | 274.6025 | 0.00045 | 275.0142 | 0.00051 |
| 274.0536 | 0.00000 | 273.3214 | 0.00039 | 274.0542 | 0.00000 | 273.3219 | 0.00609 | 274.4841 | 0.00000 | 273.8844 | 0.00457 |
| 273.9900 | 0.00059 | 273.2395 | 0.00000 | 273.9905 | 0.00526 | 273.2403 | 0.00007 | 274.4207 | 0.00040 | 273.8027 | 0.00006 |
| 273.5263 | 0.00000 | 272.8517 | 0.00000 | 273.5268 | 0.00004 | 272.8522 | 0.00000 | 273.9570 | 0.00000 | 273.4147 | 0.00000 |

Table S25: PNA: Unshifted nonresonant (XES) data at the Carbon $K$-edge for C4-C6 (the numbering is based on energies, so that first core excitation from 1s(C1) has the lowest energy) calculated using different methods. All calculations employed the 6-311++G** basis.

| C4 | | | | C5 | | | | C6 | | | |
|---|---|---|---|---|---|---|---|---|---|---|---|
| EOM-CCSD | | EOM-CC2 | | EOM-CCSD | | EOM-CC2 | | EOM-CCSD | | EOM-CC2 | |
| $\omega_{em}$/eV | $f_{osc}$ | $\omega_{em}$/eV | $f_{osc}$ | $\omega_{em}$/eV | $f_{osc}$ | $\omega_{em}$/eV | $f_{osc}$ | $\omega_{em}$/eV | $f_{osc}$ | $\omega_{em}$/eV | $f_{osc}$ |
| 284.4029 | 0.00000 | 284.2857 | 0.00000 | 284.7749 | 0.01592 | 284.3986 | 0.01552 | 285.7325 | 0.00758 | 285.6117 | 0.00634 |
| 282.9052 | 0.03094 | 283.2252 | 0.00103 | 283.2772 | 0.00000 | 283.3382 | 0.0003 | 284.2348 | 0.00000 | 284.5515 | 0.00004 |
| 282.2317 | 0.00113 | 282.8045 | 0.00113 | 282.6037 | 0.00030 | 282.9175 | 0.00610 | 283.5613 | 0.00006 | 284.1306 | 0.00001 |
| 281.9074 | 0.00075 | 282.7379 | 0.02961 | 282.2796 | 0.00000 | 282.8508 | 0.00000 | 283.2372 | 0.00000 | 284.0639 | 0.00000 |
| 281.8587 | 0.00128 | 281.9270 | 0.00125 | 282.2307 | 0.00773 | 282.0399 | 0.00000 | 283.1882 | 0.00001 | 283.2530 | 0.00000 |
| 281.0799 | 0.00000 | 281.2527 | 0.00000 | 281.4519 | 0.01417 | 281.3659 | 0.02053 | 282.4094 | 0.00315 | 282.579 | 0.00353 |
| 280.0129 | 0.00004 | 280.3131 | 0.00004 | 280.3852 | 0.00848 | 280.4260 | 0.00538 | 281.3425 | 0.01144 | 281.6391 | 0.01258 |
| 279.0360 | 0.00000 | 279.2869 | 0.00000 | 279.4080 | 0.00255 | 279.3999 | 0.00380 | 280.3656 | 0.01472 | 280.6129 | 0.01588 |
| 278.5770 | 0.00061 | 279.0088 | 0.00033 | 278.9490 | 0.00009 | 279.1218 | 0.00004 | 279.9065 | 0.00571 | 280.3351 | 0.00599 |
| 277.7609 | 0.01068 | 278.1911 | 0.01065 | 278.1329 | 0.00014 | 278.304 | 0.00646 | 279.0905 | 0.0003 | 279.5174 | 0.01077 |
| 277.6072 | 0.00925 | 278.0466 | 0.01140 | 277.9794 | 0.00917 | 278.1598 | 0.00001 | 278.9367 | 0.01035 | 279.3729 | 0.00050 |
| 277.0708 | 0.00887 | 277.3546 | 0.01002 | 277.4428 | 0.00201 | 277.4676 | 0.00294 | 278.4004 | 0.00370 | 278.6807 | 0.00541 |
| 275.8817 | 0.00003 | 276.7897 | 0.00031 | 276.2539 | 0.00047 | 276.9027 | 0.00088 | 277.2115 | 0.00034 | 278.1157 | 0.00056 |
| 275.7660 | 0.00000 | 276.0681 | 0.00000 | 276.1380 | 0.00232 | 276.181 | 0.00303 | 277.0956 | 0.00001 | 277.3941 | 0.00000 |
| 275.1326 | 0.00152 | 275.9709 | 0.00050 | 275.5048 | 0.00123 | 276.0839 | 0.00186 | 276.4624 | 0.01101 | 277.2970 | 0.00520 |
| 274.9369 | 0.00000 | 275.0738 | 0.00908 | 275.3089 | 0.00004 | 275.1867 | 0.00270 | 276.2665 | 0.00034 | 276.3998 | 0.00877 |
| 274.6049 | 0.00518 | 275.0207 | 0.00480 | 274.9769 | 0.00316 | 275.1336 | 0.00231 | 275.9345 | 0.00053 | 276.3467 | 0.00047 |
| 274.4868 | 0.00000 | 273.8912 | 0.00732 | 274.8588 | 0.00000 | 274.0041 | 0.00223 | 275.8164 | 0.00000 | 275.2172 | 0.00058 |
| 274.4232 | 0.00907 | 273.8095 | 0.00008 | 274.7951 | 0.00426 | 273.9225 | 0.00003 | 275.7527 | 0.00324 | 275.1356 | 0.00001 |
| 273.9595 | -0.00003 | 273.4215 | 0.00000 | 274.3315 | 0.00000 | 273.5344 | 0.00000 | 275.2890 | 0.00000 | 274.7475 | 0.00000 |

Table S26: PNA (6-31G basis set): Unshifted RIXS data for the pump frequency at resonance with the first bright core excitation. RIXS cross sections for $\theta = 45°$ at the CVS-EOM-CCSD and CVS-0-EOM-CCSD level of theory are both based on emission energies calculated at the EOM-CCSD level of theory. CVS and CVS-0 refer to a projection in the damped response solver. All calculations employed the 6-31G basis.

| $\omega_{em}$/eV | | $\sigma^{\text{RIXS}}_{45°}$/a.u. | | |
|---|---|---|---|---|
| CCSD | fc-CCSD | CVS-EOM-CCSD | CVS-0-EOM-CCSD | fc-CVS-0-EOM-CCSD |
| 284.7741 | 284.7319 | 0.00012 | 0.00004 | 0.00003 |
| 284.3684 | 284.3265 | 0.00126 | 0.00094 | 0.00097 |
| 284.0590 | 284.0244 | 0.00003 | 0.00000 | 0.00000 |
| 284.0255 | 283.9891 | 0.05439 | 0.01593 | 0.01656 |
| 282.5713 | 282.5332 | 0.00048 | 0.00000 | 0.00000 |
| 282.1286 | 282.0897 | 0.00005 | 0.00000 | 0.00000 |
| 281.7953 | 281.7577 | 0.00195 | 0.00197 | 0.00203 |
| 281.7477 | 281.7060 | 0.00002 | 0.00002 | 0.00002 |
| 281.0143 | 280.9795 | 0.05859 | 0.05887 | 0.06103 |
| 280.8026 | 280.7645 | 0.05633 | 0.04625 | 0.04843 |
| 280.5980 | 280.5577 | 0.00012 | 0.00014 | 0.00015 |
| 280.5237 | 280.4869 | 0.00013 | 0.00000 | 0.00000 |
| 280.4908 | 280.4543 | 0.00041 | 0.00046 | 0.00046 |
| 280.4600 | 280.4216 | 0.02193 | 0.02179 | 0.02274 |
| 280.4336 | 280.3972 | 0.10116 | 0.10114 | 0.10567 |
| 280.3610 | 280.3237 | 0.00122 | 0.00117 | 0.00093 |
| 280.2410 | 280.2012 | 0.00384 | 0.00324 | 0.00335 |
| 280.0015 | 279.9618 | 0.00038 | 0.00034 | 0.00035 |
| 279.9615 | 279.9264 | 0.00231 | 0.00226 | 0.00199 |
| 279.9188 | 279.8829 | 0.01093 | 0.01072 | 0.0116 |

## S4.3 Valence Transition NTOs

| EOM-CCSD | | | EOM-CC2 | | |
|---|---|---|---|---|---|
| Transition Symmetry | Hole NTO | Particle NTO | Transition Symmetry | Hole NTO | Particle NTO |
| $1A_1$ | 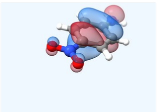 | 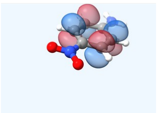 | $1A_1$ | 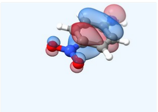 | 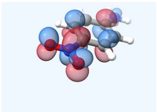 |
| $2A_1$ | 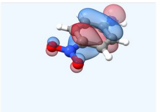 | 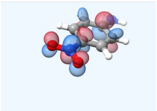 | $2A_1$ | 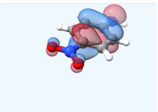 | 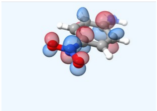 |
| $3A_1$ | 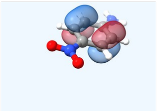 | 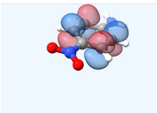 | $3A_1$ | 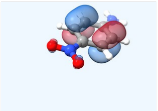 | 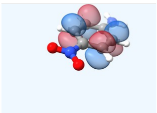 |
| $5A_1$ | 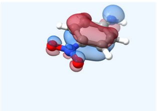 | 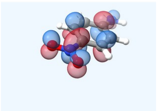 | | | |

Figure S9: PNA: NTO pairs of the probed valence transitions at both the CCSD and CC2 levels of theory using the 6-311++G** basis set. Isosurface value was 0.04 for all NTO pairs.

# S5 Imidazole

## S5.1 Treatment of solvent $H_2O$

The simulated XAS spectra in Fig. S10 (left panels) are found to correspond well with experiment. It is observed that the calculation treating the $H_2O$ molecules at the HF level of theory (top) corresponds well with that treating both solvent and solute at the CCSD level of theory (bottom). In fact, the results of two calculations are difficult to distinguish. Both calculations show a too large splitting (ca. 1.9 eV vs. the experimental of ca. 1.6 eV) as well as a slightly different intensity ratio of the main peaks. The two main transitions are found to be core $1A$ and core $2A$ in both calculations.

Considering now the valence transitions also shown in Fig. S10(left), we observe that the two methods give similar results. It is, however, noted that the valence transitions fall in a wider energy range when treating the solvent molecules at the HF-level of theory. Furthermore, this

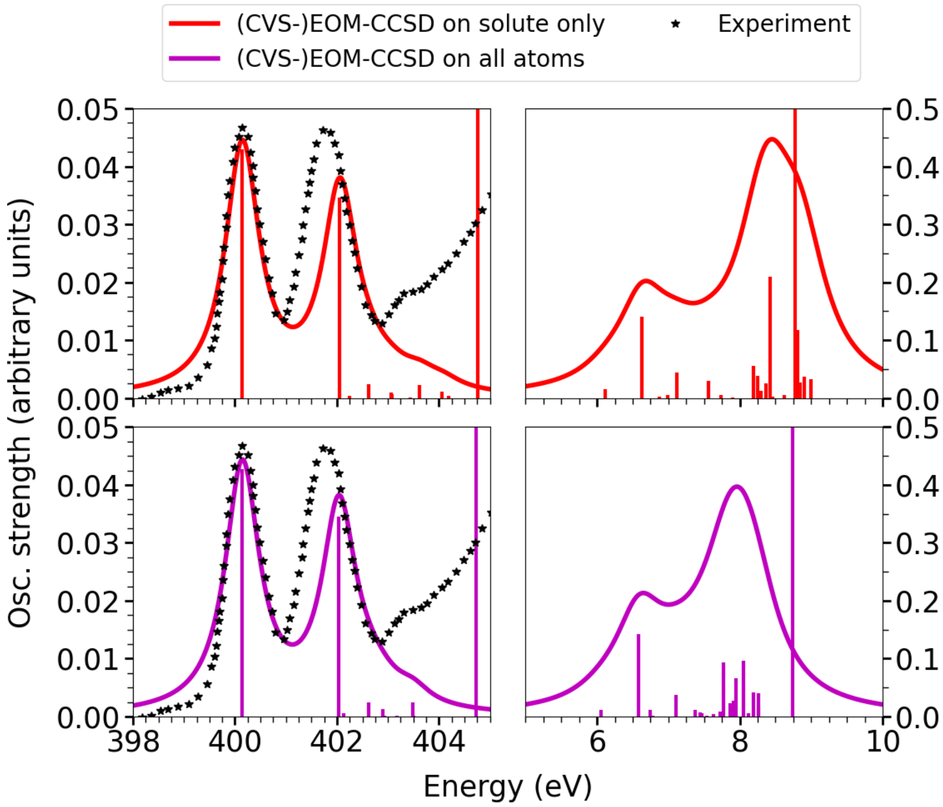


Figure S10: Imidazole with 4 explicit $H_2O$ molecules: XAS spectra at the nitrogen *K*-edge (left) and Valence absorption spectra computed in the space orthogonal to the N core space (right). All spectra were calculated at the CVS-EOM-CCSD level of theory with the 6-311++G** basis. The solvent $H_2O$ molecules are treated at the CVS-EOM-CCSD level of theory (bottom) and at the HF level of theory (top). Experimental XAS data was digitized from Meyer et al.[5] The vertical lines spanning the entire height of the plot show the first ionization threshold. The computed XAS spectra were shifted by $-1.67$ eV to align with experiment when treating all atoms at the CCSD level of theory and $-1.65$ eV when treating the solvent molecules at the HF level of theory. 10 core transitions and 20 valence transitions are shown. A Lorentzian broadening with HWHM = 0.41 eV has been applied.

treatment increases the intensities of the two main transitions of the high energy peak. Despite these differences at higher transition energies, we find that the significantly cheaper approach of treating the solvent molecules at the HF-level of theory is sufficient when it comes to describing also the more delocalized valence transitions.

## S5.2 Solvent $H_2O$ treated at the CCSD level of theory

As also seen in the main text, as well as in Meyer et al.,[5] the RIXS spectra at the two first resonances can be compared to the nonresonant spectra for each individual nitrogen. This can be seen in Fig. S11. It is observed that the RIXS spectrum for the first core resonance shows good agreement with the XES spectrum calculated for N1, while the signal at the second core resonance agrees well with the XES spectrum computed for N3.

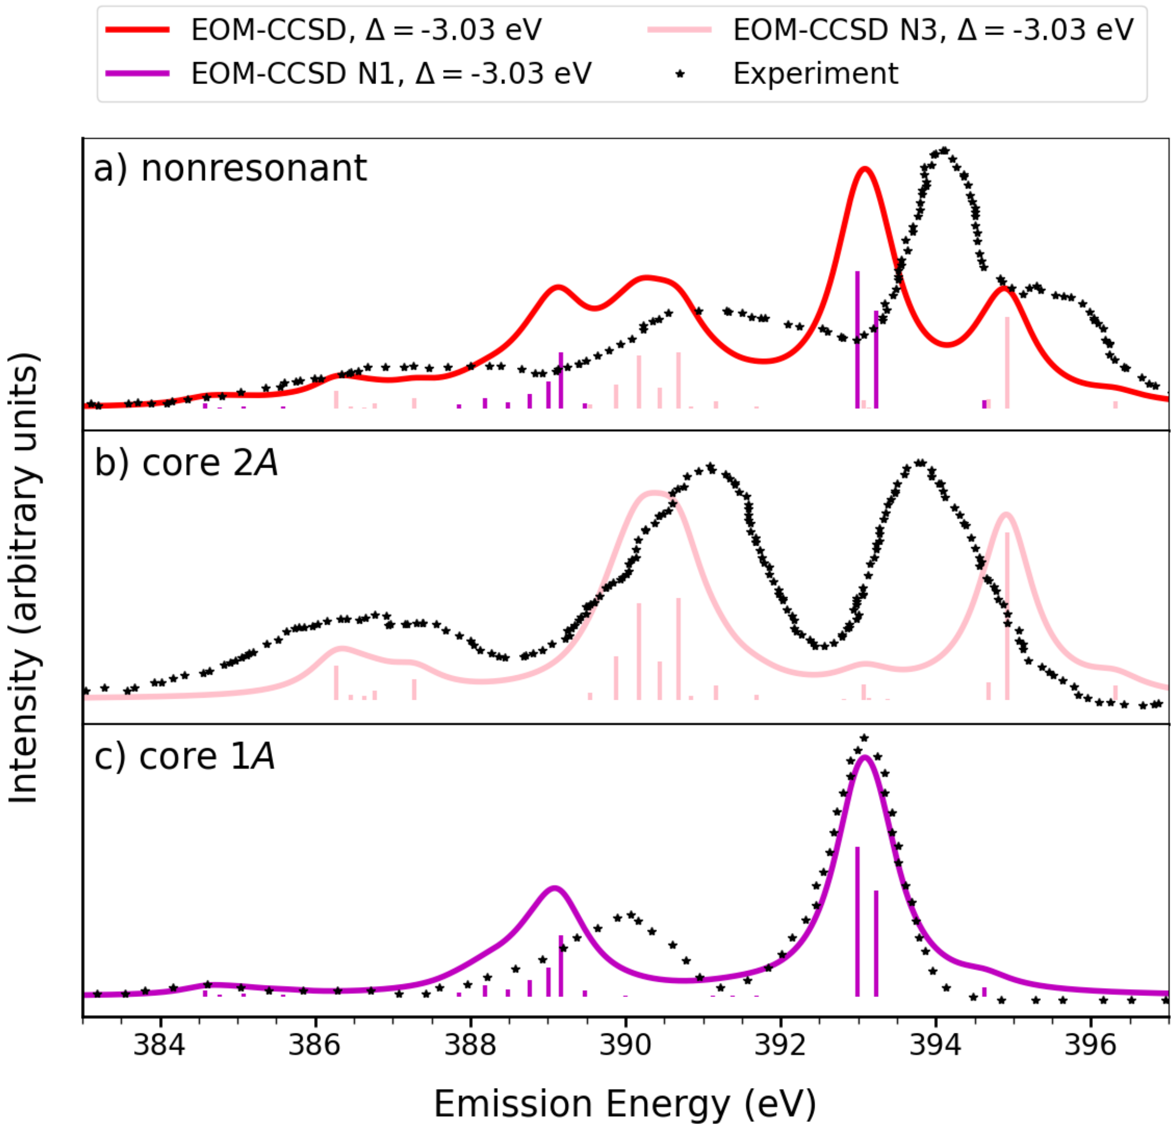


Figure S11: Imidazole with 4 explicit $H_2O$ molecules: Nonresonant (a) and RIXS spectra at resonance with the energy of the first (c), and second (b) core excitation at the N *K*-edge. All spectra are computed with the 6-311++G** basis at the EOM-CCSD level of theory for both solute and solvent. The results are shifted based on the RIXS experiment at resonance with the first core excitation. A Lorentzian broadening of the spectra have been applied with HWHM=0.41 eV. For (b) and (c) the simulated spectra are the nonresonant ones of individual N-atoms as indicated in the legends. Experimental data was digitized from Meyer et al.[5]

### S5.2.1 Data tables

Table S27: Imidazole with 4 explicit $H_2O$ molecules: Unshifted N $K$-edge XAS data using the 6-311++G** basis set at the CVS-EOM-CCSD level of theory for all atoms.

| Sym.[a] | $\omega_{abs,c}$/eV | $f_{osc}$ |
|---|---|---|
| 1*A* | 401.8125 | 0.04270 |
| 2*A* | 403.7078 | 0.03452 |
| 3*A* | 403.799 | 0.00057 |
| 4*A* | 404.282 | 0.00242 |
| 5*A* | 404.5691 | 0.00133 |
| 6*A* | 404.6025 | 0.00021 |
| 7*A* | 404.8462 | 0.00007 |
| 8*A* | 405.1582 | 0.00238 |
| 9*A* | 405.1664 | 0.00014 |
| 10*A* | 405.3222 | 0.00001 |

[a] Mulliken symmetry notation.

Table S28: Imidazole with 4 explicit $H_2O$ molecules: Unshifted valence excitation data computed using the 6-311++G** basis set in a space orthogonal to the N core space. For solute as well as solvent the EOM-CCSD level of theory was used.

| Sym.[a] | $\omega_{abs,v}$/eV | $f_{osc}$ |
|---|---|---|
| 1*A* | 6.0528 | 0.01210 |
| 2*A* | 6.5819 | 0.14179 |
| 3*A* | 6.7463 | 0.01116 |
| 4*A* | 6.7841 | 0.00122 |
| 5*A* | 7.1072 | 0.03736 |
| 6*A* | 7.3754 | 0.01150 |
| 7*A* | 7.4410 | 0.00719 |
| 8*A* | 7.4629 | 0.00566 |
| 9*A* | 7.5410 | 0.00147 |
| 10*A* | 7.6324 | 0.00384 |
| 11*A* | 7.7305 | 0.00817 |
| 12*A* | 7.7752 | 0.09371 |
| 13*A* | 7.8601 | 0.02239 |
| 14*A* | 7.9173 | 0.02735 |
| 15*A* | 7.9454 | 0.06602 |
| 16*A* | 8.0535 | 0.09648 |
| 17*A* | 8.1198 | 0.00562 |
| 18*A* | 8.1901 | 0.04189 |
| 19*A* | 8.2559 | 0.01930 |
| 20*A* | 8.2657 | 0.04033 |

[a] Mulliken symmetry notation.

Table S29: Imidazole with 4 explicit $H_2O$ molecules: Unshifted nonresonant (XES) data at the Nitrogen $K$-edge for N1 and N3 calculated using EOM-CCSD on both solute and solvent. All calculations employed the 6-311++G** basis.

| N1 | | N3 | |
|---|---|---|---|
| $\omega_{em}$/eV | $f_{osc}$ | $\omega_{em}$/eV | $f_{osc}$ |
| 397.6639 | 0.00230 | 399.3504 | 0.00195 |
| 396.2693 | 0.02449 | 397.9558 | 0.02294 |
| 396.0293 | 0.03446 | 397.7158 | 0.00236 |
| 394.7256 | 0.00019 | 396.4121 | 0.00016 |
| 394.4897 | 0.00014 | 396.1762 | 0.00030 |
| 394.4148 | 0.00017 | 396.1014 | 0.00214 |
| 394.1577 | 0.00017 | 395.8442 | 0.00006 |
| 393.0322 | 0.00023 | 394.7188 | 0.00075 |
| 392.5157 | 0.00137 | 394.2023 | 0.00197 |
| 392.1982 | 0.01407 | 393.8847 | 0.00061 |
| 392.0376 | 0.00679 | 393.7242 | 0.01400 |
| 391.7960 | 0.00376 | 393.4826 | 0.00528 |
| 391.5244 | 0.00174 | 393.2110 | 0.01329 |
| 391.2216 | 0.00279 | 392.9081 | 0.00595 |
| 390.8912 | 0.00109 | 392.5775 | 0.00103 |
| 388.6267 | 0.00054 | 390.3132 | 0.00278 |
| 388.1184 | 0.00072 | 389.8049 | 0.00128 |
| 387.9875 | 0.00012 | 389.6741 | 0.00050 |
| 387.8025 | 0.00044 | 389.4890 | 0.00070 |
| 387.6180 | 0.00142 | 389.3045 | 0.00463 |

## S5.3 Solvent $H_2O$ treated at HF level of theory

To save computational power we have treated the solvent molecules at the HF level of theory and only employ CCSD for the imidazole molecule itself. This approach was shown in section S5.1 to work excellently for the localized core transitions, and even for the more delocalized valence transitions did the method yield good results.

As the method is computationally cheaper compared to treating both solvent and solute at the CCSD level of theory, more valence transitions can be considered. The corresponding valence absorption spectrum is shown in Fig. S12

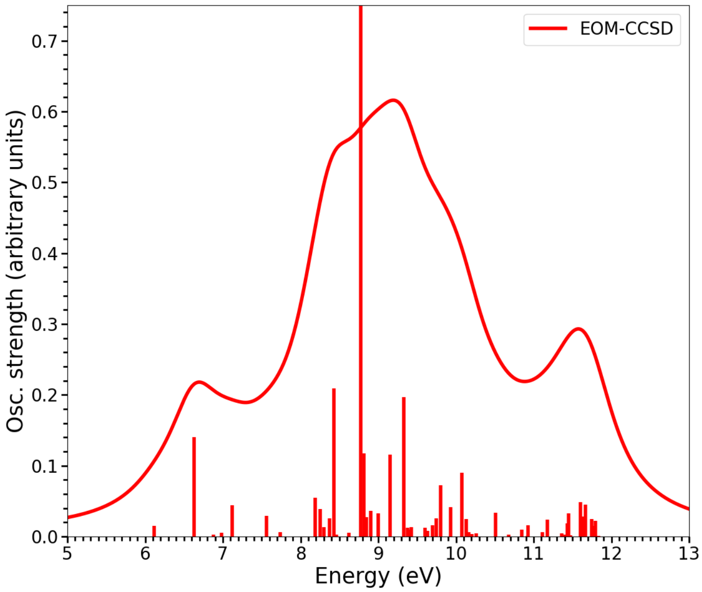


Figure S12: Imidazole with 4 explicit $H_2O$ molecules, the latter treated at the HF level of theory: Valence absorption spectrum computed in the space orthogonal to the N core space and calculated at the EOM-CCSD (red) level of theory with the 6-311++G** basis. The vertical line spanning the entire height of the plot shows the first ionization threshold. A Lorentizian broadening was applied with HWHM=0.41 eV. 60 valence transitions are shown.

### S5.3.1 Data tables

Table S30: Imidazole with 4 explicit $H_2O$ molecules, the latter treated at the HF level of theory: Unshifted N $K$-edge XAS data using the 6-311++G** basis set and CVS-EOM-CCSD method.
[a] Mulliken symmetry notation.

| Sym.[a] | $\omega_{abs,c}$/eV | $f_{osc}$ |
|---|---|---|
| 1$A$ | 401.7992 | 0.04291 |
| 2$A$ | 403.7125 | 0.03463 |
| 3$A$ | 403.9067 | 0.00038 |
| 4$A$ | 404.2742 | 0.00242 |
| 5$A$ | 404.7165 | 0.00100 |
| 6$A$ | 404.7382 | 0.00063 |
| 7$A$ | 405.1006 | 0.00002 |
| 8$A$ | 405.2667 | 0.00224 |
| 9$A$ | 405.7138 | 0.00116 |
| 10$A$ | 405.8489 | 0.00032 |

Table S31: Imidazole with 4 explicit $H_2O$ molecules, the latter treated at the HF level of theory: Unshifted valence absorption data computed using the 6-311++G** basis set in a space orthogonal to the N core space at the EOM-CCSD level of theory.
[a] Mulliken symmetry notation.

| Sym.[a] | $\omega_{abs,v}$/eV | $f_{osc}$ |
|---|---|---|
| 1*A* | 6.1192 | 0.01508 |
| 2*A* | 6.6315 | 0.13996 |
| 3*A* | 6.8779 | 0.00300 |
| 4*A* | 6.9847 | 0.00542 |
| 5*A* | 7.1231 | 0.04414 |
| 6*A* | 7.5644 | 0.02921 |
| 7*A* | 7.6314 | 0.00011 |
| 8*A* | 7.7390 | 0.00589 |
| 9*A* | 7.9027 | 0.00024 |
| 10*A* | 8.1887 | 0.05492 |
| 11*A* | 8.2551 | 0.03864 |
| 12*A* | 8.2980 | 0.01294 |
| 13*A* | 8.3718 | 0.02535 |
| 14*A* | 8.4288 | 0.20931 |
| 15*A* | 8.4633 | 0.00245 |
| 16*A* | 8.6246 | 0.00490 |
| 17*A* | 8.8134 | 0.11727 |
| 18*A* | 8.8470 | 0.02711 |
| 19*A* | 8.9051 | 0.03635 |
| 20*A* | 8.9965 | 0.03226 |
| 21*A* | 9.1495 | 0.11523 |
| 22*A* | 9.3329 | 0.19650 |
| 23*A* | 9.3756 | 0.01266 |
| 24*A* | 9.4043 | 0.00928 |
| 25*A* | 9.4265 | 0.01289 |
| 26*A* | 9.6032 | 0.01259 |
| 27*A* | 9.6308 | 0.00754 |
| 28*A* | 9.6997 | 0.01580 |
| 29*A* | 9.7434 | 0.02551 |
| 30*A* | 9.8054 | 0.07274 |
| 31*A* | 9.9284 | 0.04141 |
| 32*A* | 10.0725 | 0.09012 |
| 33*A* | 10.1290 | 0.02495 |
| 34*A* | 10.1644 | 0.00592 |

**Table S31 – continued from previous page**

| Sym.[a] | $\omega_{abs,v}$/eV | $f_{osc}$ |
|---|---|---|
| 35*A* | 10.2028 | 0.00328 |
| 36*A* | 10.2592 | 0.00451 |
| 37*A* | 10.5134 | 0.03315 |
| 38*A* | 10.5817 | 0.00025 |
| 39*A* | 10.6768 | 0.00235 |
| 40*A* | 10.8473 | 0.00966 |
| 41*A* | 10.9200 | 0.00131 |
| 42*A* | 10.9296 | 0.01611 |
| 43*A* | 11.0170 | 0.00001 |
| 44*A* | 11.1113 | 0.00657 |
| 45*A* | 11.1739 | 0.00038 |
| 46*A* | 11.1805 | 0.02356 |
| 47*A* | 11.3593 | 0.00398 |
| 48*A* | 11.4035 | 0.00230 |
| 49*A* | 11.4089 | 0.00264 |
| 50*A* | 11.4300 | 0.01816 |
| 51*A* | 11.4510 | 0.03238 |
| 52*A* | 11.4711 | 0.00165 |
| 53*A* | 11.6061 | 0.04848 |
| 54*A* | 11.6326 | 0.02827 |
| 55*A* | 11.6685 | 0.04525 |
| 56*A* | 11.7457 | 0.02432 |
| 57*A* | 11.7758 | 0.01495 |
| 58*A* | 11.7916 | 0.02203 |
| 59*A* | 11.8108 | 0.00115 |
| 60*A* | 11.8383 | 0.00102 |

Table S32: Imidazole with 4 explicit $H_2O$ molecules, the latter treated at the HF level of theory: Unshifted RIXS data for the pump frequency at resonance with the first bright core excitation (1*A* in Mulliken symmetry notation) calculated using different CCSD methods. All computed RIXS cross sections for $\theta = 45^\circ$ are based on emission energies calculated at the EOM-CCSD level of theory. CVS and CVS-uS refer to a projection in the damped response solver. All calculations employed the 6-311++G** basis.

| $\omega_{em}$/eV | $\sigma^{\text{RIXS}}_{45^\circ}$/a.u. | |
|---|---|---|
| CCSD | CVS-uS-EOM-CCSD | CVS-EOM-CCSD |
| 395.6799 | 0.00008 | 0.00134 |
| 395.1678 | 0.00116 | 0.00166 |
| 394.9212 | 0.00007 | 0.00031 |

**Table S32 – continued from previous page**

| $\omega_{em}$/eV | $\sigma_{45^\circ}^{\text{RIXS}}$/a.u. | |
|---|---|---|
| CCSD | CVS-uS-EOM-CCSD | CVS-EOM-CCSD |
| 394.8146 | 0.00029 | 0.00032 |
| 394.6761 | 0.00576 | 0.00621 |
| 394.2347 | 0.00078 | 0.00158 |
| 394.1677 | 0.00116 | 0.00152 |
| 394.0603 | 0.08221 | 0.06826 |
| 393.8964 | 0.00047 | 0.00099 |
| 393.6105 | 0.00010 | 0.00009 |
| 393.5441 | 0.00107 | 0.00077 |
| 393.5013 | 0.00029 | 0.00033 |
| 393.4273 | 0.00017 | 0.00018 |
| 393.3704 | 0.01376 | 0.01199 |
| 393.3359 | 0.00020 | 0.00027 |
| 393.1745 | 0.01861 | 0.01545 |
| 392.9857 | 0.00156 | 0.00174 |
| 392.9522 | 0.00063 | 0.00126 |
| 392.8942 | 0.00151 | 0.00385 |
| 392.8028 | 0.00076 | 0.00070 |
| 392.6496 | 0.00473 | 0.00462 |
| 392.4662 | 0.00518 | 0.00458 |
| 392.4235 | 0.00070 | 0.00058 |
| 392.3949 | 0.00047 | 0.00025 |
| 392.3729 | 0.00083 | 0.00069 |
| 392.1960 | 0.00031 | 0.00011 |
| 392.1682 | 0.00025 | 0.00029 |
| 392.0994 | 0.00031 | 0.00030 |
| 392.0559 | 0.00003 | 0.00010 |
| 391.9938 | 0.00014 | 0.00021 |
| 391.8708 | 0.00007 | 0.00026 |
| 391.7269 | 0.00009 | 0.00009 |
| 391.6703 | 0.00007 | 0.00023 |
| 391.6349 | 0.00007 | 0.00006 |
| 391.5965 | 0.00007 | 0.00007 |
| 391.5399 | 0.00014 | 0.00039 |
| 391.2858 | 0.00002 | 0.00137 |
| 391.2175 | 0.00012 | 0.00060 |
| 391.1225 | 0.00008 | 0.00013 |
| 390.9519 | 0.00448 | 0.00395 |
| 390.8792 | 0.00013 | 0.00014 |

Table S32 – continued from previous page

| $\omega_{em}$/eV | $\sigma^{\mathrm{RIXS}}_{45^\circ}$/a.u. | |
|---|---|---|
| CCSD | CVS-uS-EOM-CCSD | CVS-EOM-CCSD |
| 390.8697 | 0.00010 | 0.00012 |
| 390.7821 | 0.00056 | 0.00048 |
| 390.6879 | 0.00005 | 0.00003 |
| 390.6254 | 0.01555 | 0.01322 |
| 390.6188 | 0.01506 | 0.01283 |
| 390.4401 | 0.00061 | 0.00058 |
| 390.3957 | 0.00031 | 0.00053 |
| 390.3903 | 0.00098 | 0.00085 |
| 390.3693 | 0.00326 | 0.00293 |
| 390.3483 | 0.00298 | 0.00288 |
| 390.3282 | 0.00036 | 0.00033 |
| 390.1932 | 0.00018 | 0.00022 |
| 390.1666 | 0.00008 | 0.00007 |
| 390.1307 | 0.00001 | 0.00022 |
| 390.0534 | 0.00068 | 0.00055 |
| 390.0234 | 0.00011 | 0.00020 |

Table S33: Imidazole with 4 explicit $H_2O$ molecules, the latter treated at the HF level of theory: Unshifted RIXS data for the pump frequency at resonance with the second bright core excitation (2*A* in Mulliken symmetry notation) calculated using different CCSD methods. All computed RIXS cross sections for $\theta = 45^\circ$ are based on emission energies calculated at the EOM-CCSD level of theory. CVS and CVS-uS refer to a projection in the damped response solver. All calculations employed the 6-311++G** basis.

| $\omega_{em}$/eV | $\sigma^{\mathrm{RIXS}}_{45^\circ}$/a.u. | |
|---|---|---|
| CCSD | CVS-uS-EOM-CCSD | CVS-EOM-CCSD |
| 397.5931 | 0.00007 | 0.00137 |
| 397.0810 | 0.00366 | 0.00400 |
| 396.8345 | 0.00006 | 0.00027 |
| 396.7278 | 0.00025 | 0.00029 |
| 396.5893 | 0.00639 | 0.00668 |
| 396.1479 | 0.00117 | 0.00188 |
| 396.0810 | 0.00017 | 0.00091 |
| 395.9735 | 0.00621 | 0.00541 |
| 395.8097 | 0.00009 | 0.00069 |
| 395.5237 | 0.00019 | 0.00020 |
| 395.4573 | 0.00075 | 0.00048 |
| 395.4146 | 0.00019 | 0.00025 |

**Table S33 – continued from previous page**

| $\omega_{em}$/eV | $\sigma^{\mathrm{RIXS}}_{45^\circ}$/a.u. | |
|---|---|---|
| CCSD | CVS-uS-EOM-CCSD | CVS-EOM-CCSD |
| 395.3406 | 0.00041 | 0.00038 |
| 395.2837 | 0.01347 | 0.01160 |
| 395.2491 | 0.00017 | 0.00029 |
| 395.0878 | 0.00063 | 0.00058 |
| 394.8989 | 0.00091 | 0.00133 |
| 394.8654 | 0.00008 | 0.00097 |
| 394.8075 | 0.00110 | 0.00352 |
| 394.7161 | 0.00008 | 0.00019 |
| 394.5629 | 0.00005 | 0.00058 |
| 394.3794 | 0.00345 | 0.00305 |
| 394.3367 | 0.00047 | 0.00037 |
| 394.3082 | 0.00036 | 0.00017 |
| 394.2861 | 0.00008 | 0.00014 |
| 394.1092 | 0.00029 | 0.00010 |
| 394.0815 | 0.00016 | 0.00019 |
| 394.0126 | 0.00019 | 0.00018 |
| 393.9691 | 0.00003 | 0.00010 |
| 393.9071 | 0.00011 | 0.00020 |
| 393.7841 | 0.00009 | 0.00028 |
| 393.6401 | 0.00007 | 0.00007 |
| 393.5835 | 0.00008 | 0.00026 |
| 393.5481 | 0.00010 | 0.00008 |
| 393.5098 | 0.00006 | 0.00007 |
| 393.4532 | 0.00030 | 0.00055 |
| 393.1990 | 0.00001 | 0.00137 |
| 393.1307 | 0.00009 | 0.00056 |
| 393.0357 | 0.00000 | 0.00003 |
| 392.8651 | 0.00054 | 0.00077 |
| 392.7925 | 0.00003 | 0.00005 |
| 392.7830 | 0.00020 | 0.00019 |
| 392.6953 | 0.00006 | 0.00009 |
| 392.6012 | 0.00021 | 0.00016 |
| 392.5386 | 0.00160 | 0.00132 |
| 392.5321 | 0.00131 | 0.00110 |
| 392.3533 | 0.00169 | 0.00146 |
| 392.3089 | 0.00129 | 0.00140 |
| 392.3035 | 0.00394 | 0.00337 |
| 392.2825 | 0.00840 | 0.00727 |

Table S33 – continued from previous page

| $\omega_{em}$/eV | $\sigma^{\text{RIXS}}_{45^\circ}$/a.u. | |
|---|---|---|
| CCSD | CVS-uS-EOM-CCSD | CVS-EOM-CCSD |
| 392.2616 | 0.00742 | 0.00667 |
| 392.2414 | 0.00016 | 0.00017 |
| 392.1065 | 0.00090 | 0.00083 |
| 392.0798 | 0.00182 | 0.00160 |
| 392.0439 | 0.00010 | 0.00029 |
| 391.9669 | 0.00434 | 0.00383 |
| 391.9367 | 0.00209 | 0.00193 |

Table S34: Imidazole with 4 explicit $H_2O$ molecules, the latter treated at the HF level of theory: Unshifted nonresonant (XES) data at the Nitrogen $K$-edge calculated using EOM-CCSD for N1 and N3 using the 6-311++G** basis.

| N1 | | N3 | |
|---|---|---|---|
| $\omega_{em}$/eV | $f_{osc}$ | $\omega_{em}$/eV | $f_{osc}$ |
| 397.6367 | 0.00221 | 399.3420 | 0.00197 |
| 396.2244 | 0.02475 | 397.9297 | 0.02302 |
| 395.7863 | 0.03618 | 397.4916 | 0.00267 |
| 393.3944 | 0.00010 | 395.1000 | 0.00266 |
| 392.2205 | 0.01403 | 393.9258 | 0.00054 |
| 391.9761 | 0.00771 | 393.6815 | 0.01598 |
| 391.5979 | 0.00620 | 393.3035 | 0.00902 |
| 391.3995 | 0.00287 | 393.1049 | 0.01633 |
| 390.5367 | 0.00033 | 392.2423 | 0.00053 |
| 387.9146 | 0.00237 | 389.6199 | 0.01064 |
| 387.2462 | 0.00000 | 388.9519 | 0.00047 |
| 387.1453 | 0.00070 | 388.8506 | 0.01216 |
| 386.6658 | 0.00659 | 388.3712 | 0.0117 |
| 386.2228 | 0.00018 | 387.9282 | 0.0000 |
| 385.5110 | 0.00010 | 387.2163 | 0.00028 |
| 385.3850 | 0.00000 | 387.0903 | 0.00001 |
| 385.1553 | 0.00000 | 386.8609 | 0.00000 |
| 384.9970 | 0.00000 | 386.7023 | 0.00010 |
| 384.8204 | 0.00000 | 386.5257 | 0.00001 |
| 384.5953 | 0.00001 | 386.3007 | 0.00001 |

# S6 Pyridine

Another example molecule simulated with the new implementation is pyridine. The simulated XAS spectrum at the nitrogen K-edge is shown in Fig. S13. The CVS-EOM-CCSD result is observed to be in good agreement with the experimental spectrum, and is further more noted to be an improvement on the simulated DFT spectra shown in.[6] The lack of the small shoulder on the main peak is expected, as this is reported to be the result of a dipole forbidden transition

only allowed through vibronic coupling,[6] which is not included in this study. It can be seen from

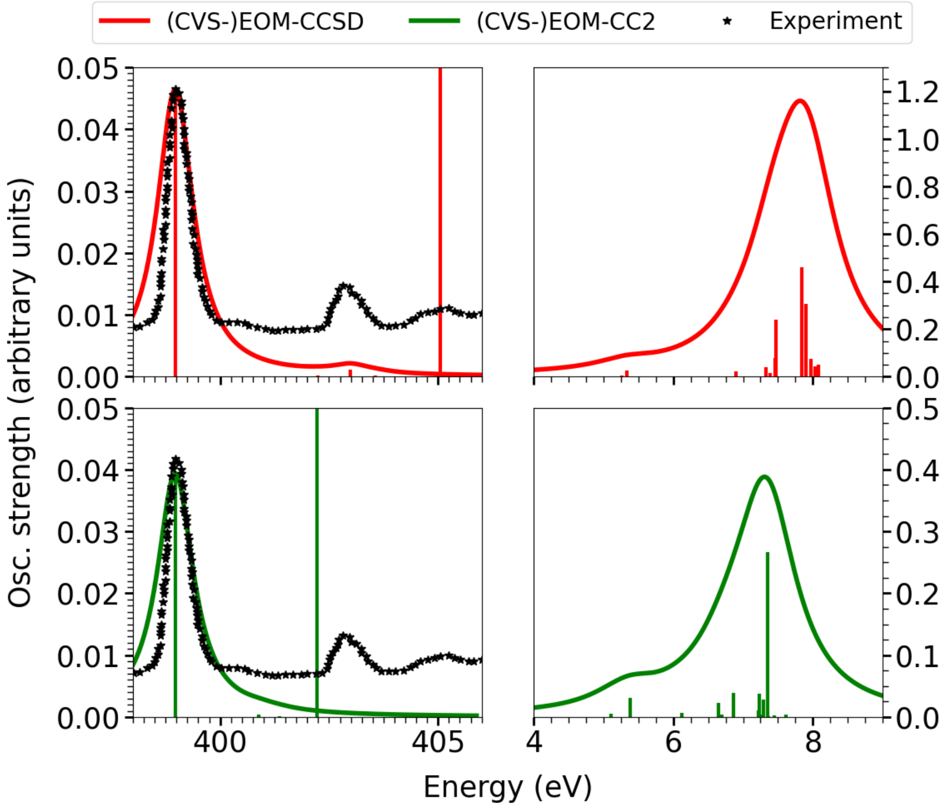


Figure S13: Pyridine: XAS spectrum at the nitrogen $K$-edge (left) and valence absorption in a space orthogonal to the N core space (right) calculated at the (CVS-)EOM-CC2 (green) and (CVS-)EOM-CCSD (red) level of theory with the 6-311++G** basis including additional Rydberg functions on N. Experimental data was digitized from Baiardi et al..[6] The vertical lines spanning the entire height of the plot shows the first (core) ionization threshold. The Lorentizian broadening applied has HWHM=0.51 eV. The computed XAS were shifted to align with experiment: $-1.69$ eV for CVS-EOM-CCSD and $-2.28$ eV for CVS-EOM-CC2.

Fig. S13 that CVS-EOM-CC2 predicts the second (low intensity) peak far closer to the first peak compared to CVS-EOM-CCSD and experiment. Furthermore, this second feature at the CVS-EOM-CC2 level of theory shows even lower intensity compared to CVS-EOM-CCSD, which also shows a too low relative intensity of the second peak compared to experiment. The core ionization threshold with CC2 is predicted to be significantly lower than what is found with CCSD, which appears to be in better general agreement with experiment (if the shift applied in Fig. S13 is considered). The characters of the two main transition are for both methods core $1A''$ and core $3A'$, respectively. The ionization thresholds are shown in table S35. From the valence spectra in Fig.

Table S35: Pyridine: Valence and core ionization energies. All calculations employed the 6-311++G** basis on all atoms with additional Rydberg functions on N.

| Method | IP/eV | Core IP/eV |
|---|---|---|
| EOM-CC2 | 9.35 | 404.50 |
| EOM-CCSD | 9.68 | 406.74 |
| Experiment[7,8] | 9.34 | 404.94 |

S13, it can be seen that, while the same overall shape is found for the two methods, a much larger intensity of the main peak is predicted by EOM-CCSD compared to EOM-CC2. This is caused by a much higher density of transitions around the main peak in the EOM-CCSD calculation. The main transition has $9A'$ character in the EOM-CC2 calculation, while it has $7A'$ character in the EOM-CCSD one.

The nonresonant as well as RIXS spectra have been computed at the resonance of the first two bright core transitions. Observe that it was not possible to converge the damped response equations for EOM-CC2, and hence the CC2 based RIXS spectrum is here CVS-uS-EOM-CC2. This might be related to the damped response solver being solved in full space in the current implementation.

The RIXS spectrum in Fig. S14, shows 3 features at the first resonance, when utilizing CCSD

Table S36: Pyridine: Overview of valence states probed in RIXS with the different methods at the first and second core resonance. The Mulliken symmetry notation has been used. All energies are unshifted.

| CVS-us-EOM-CCSD | | CVS-EOM-CCSD | | CVS-us-EOM-CC2 | |
|---|---|---|---|---|---|
| Energy/ eV | Probed state | Energy/ eV | Probed state | Energy/ eV | Probed state |
| core $1A''$ resonance | | | | | |
| 395.40 | $1A''$ | 395.40 | $1A''$ | 396.15 | $1A''$ |
| 393.75 | $3A'$ | 393.75 | $3A'$ | 394.39 | $5A'$ |
| 392.82 | $7A'$ | 392.82 | $7A'$ | - | - |
| core $3A'$ resonance | | | | | |
| - | - | - | - | 398.06 | $1A''$ |
| - | - | 397.90 | $3A''$ | | |
| 397.23 | $5A'$ | 397.23 | $5A'$ | | |
| - | - | 396.60 | $11A'$ | - | - |
| - | - | - | - | 396.47 | $4A'$ |

based methods and only 2 when considering the CC2 based one. Both the CVS-EOM-CCSD and CVS-uS-EOM-CCSD results show the same features in the same positions and probe the valence

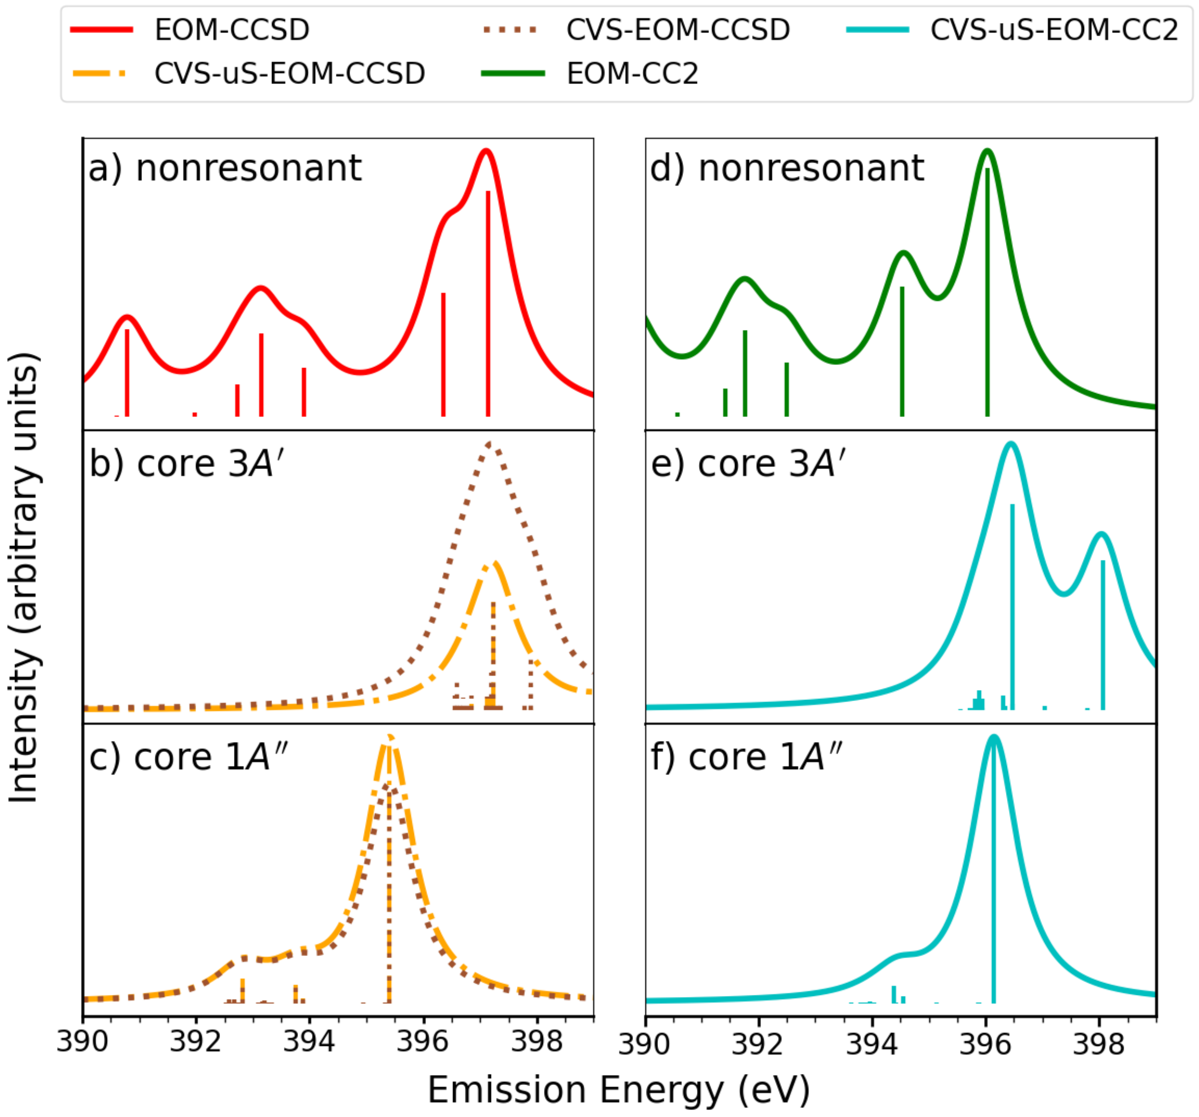


Figure S14: Pyridine: Nonresonant (a) and RIXS spectra at resonance with the energy of the first (c), and second (b) core excitation at the N *K*-edge. All spectra are computed with the 6-311++G** basis including additional Rydberg functions on N. The Lorentizian broadening applied has HWHM=0.51 eV.

$1A''$, $3A'$ and $7A'$ transitions, while the CVS-uS-EOM-CC2 simulation probes only the $1A''$ and $5A'$ transitions. Comparing the CCSD and CC2 based results it is found that the first two features are described by all methods and with roughly the same separation despite the difference in the character of the second (low intensity) peak.

As also observed for the other molecules, the shift applied to align the spectra with the RIXS spectrum at the first core resonance does not overlay the CCSD and CC2 based results for the nonresonant spectra, but rather an additional shift is observed. It is furthermore noted, that while all calculations agree on the general shape of the spectra for the nonresonant spectrum as well as the RIXS spectrum at the first core resonance, there is a larger discrepancy at the second core resonance (core $3A'$). While, the CVS-EOM-CCSD spectrum shows three main transitions resulting in one broad peak, probing the valence states $5A'$, $3A''$ and $11A'$, the CVS-uS-EOM-CCSD spectrum shows only one main transition probing $5A'$. The CVS-uS-EOM-CC2 result shows yet another spectral shape and appears to probe valence transitions $1A''$ and $4A'$.

## S6.1 Data Tables

Table S37: Pyridine: Unshifted N $K$-edge XAS data using the 6-311++G** basis set with additional Rydberg functions on N.
[a] Mulliken symmetry notation.

| EOM-CC2 | | | EOM-CCSD | | |
|---|---|---|---|---|---|
| Sym.[a] | $\omega_{abs,c}$/eV | $f_{osc}$ | Sym.[a] | $\omega_{abs,c}$/eV | $f_{osc}$ |
| $1A''$ | 401.2539 | 0.03933 | $1A''$ | 400.6602 | 0.04639 |
| $2A''$ | 402.2851 | 0.00000 | $2A''$ | 402.8414 | 0.00000 |
| $1A'$ | 402.6349 | 0.00000 | $1A'$ | 403.9262 | 0.00015 |
| $2A'$ | 403.0715 | 0.00000 | $2A'$ | 404.5937 | 0.00000 |
| $3A'$ | 403.1699 | 0.00044 | $3A''$ | 404.6680 | 0.00012 |
| $3A''$ | 403.2020 | 0.00001 | $3A'$ | 404.6858 | 0.00116 |
| $4A'$ | 403.5812 | 0.00003 | $4A'$ | 405.0469 | 0.00001 |
| $5A'$ | 403.6243 | 0.00005 | $5A'$ | 405.2475 | 0.00009 |
| $6A'$ | 403.6554 | 0.00009 | $6A'$ | 405.2568 | 0.00014 |
| $4A''$ | 403.6918 | 0.00000 | $4A''$ | 405.3636 | 0.00000 |

Table S38: Pyridine: Unshifted valence absorption data computed using the 6-311++G** basis set with additional Rydberg functions on N in a space orthogonal to the N core space.
[a] Mulliken symmetry notation.

| EOM-CC2 | | | EOM-CCSD | | |
|---|---|---|---|---|---|
| Sym.[a] | $\omega_{abs,v}$/eV | $f_{osc}$ | Sym.[a] | $\omega_{abs,v}$/eV | $f_{osc}$ |
| $1A''$ | 5.1037 | 0.00574 | $1A''$ | 5.2561 | 0.00594 |
| $2A''$ | 5.3701 | 0.00000 | $1A'$ | 5.3357 | 0.02726 |
| $1A'$ | 5.3816 | 0.03091 | $2A''$ | 5.7078 | 0.00000 |
| $2A'$ | 6.1211 | 0.00632 | $2A'$ | 6.7854 | 0.00262 |
| $3A'$ | 6.6432 | 0.0224 | $3A''$ | 6.7864 | 0.00000 |
| $4A'$ | 6.6966 | 0.00385 | $3A'$ | 6.9009 | 0.02303 |
| $3A''$ | 6.6971 | 0.00000 | $4A''$ | 7.3326 | 0.04090 |
| $4A''$ | 6.8249 | 0.00066 | $4A'$ | 7.3874 | 0.01433 |
| $5A'$ | 6.8637 | 0.03945 | $5A'$ | 7.4557 | 0.07883 |
| $6A'$ | 7.2215 | 0.01121 | $6A'$ | 7.4717 | 0.24066 |
| $5A''$ | 7.2286 | 0.0382 | $5A''$ | 7.4870 | 0.00026 |
| $7A'$ | 7.2515 | 0.0043 | $6A''$ | 7.5540 | 0.00303 |
| $8A'$ | 7.2899 | 0.02854 | $7A''$ | 7.5711 | 0.00000 |
| $9A'$ | 7.3525 | 0.26711 | $7A'$ | 7.8417 | 0.46036 |
| $6A''$ | 7.3600 | 0.00096 | $8A'$ | 7.901 | 0.30515 |
| $7A''$ | 7.4114 | 0.00000 | $8A''$ | 7.9341 | 0.00000 |
| $10A'$ | 7.4341 | -0.00002 | $9A'$ | 7.9778 | 0.07613 |
| $8A''$ | 7.4459 | 0.00252 | $10A'$ | 8.0367 | 0.04440 |
| $9A''$ | 7.4478 | 0.00000 | $11A'$ | 8.0854 | 0.05158 |
| $11A'$ | 7.6111 | 0.00442 | $9A''$ | 8.1321 | 0.00018 |

Table S39: Pyridine: Unshifted RIXS data for the pump frequency at resonance with the first core excitation (core $1A''$ in Mulliken symmetry notation) calculated using different methods. RIXS cross sections for $\theta = 45°$ at the CVS-uS-EOM-CCSD and CVS-EOM-CCSD level of theory are all based on emission energies calculated at the EOM-CCSD level of theory. CVS and CVS-uS refer to a projection in the damped response solver. All calculations employed the 6-311++G** basis with additional Rydberg functions on N.

| $\omega_{em}$/eV | | $\sigma^{\mathrm{RIXS}}_{45°}$/a.u. | | |
|---|---|---|---|---|
| CCSD | CC2 | CVS-uS-EOM-CCSD | CVS-EOM-CCSD | CVS-uS-EOM-CC2 |
| 395.4040 | 396.1501 | 0.10524 | 0.08637 | 0.09736 |
| 395.3245 | 395.8837 | 0.00000 | 0.00001 | 0.00003 |
| 394.9522 | 395.8723 | 0.00003 | 0.00001 | 0.00000 |
| 393.8747 | 395.1327 | 0.00176 | 0.00190 | 0.00001 |
| 393.8739 | 394.6107 | 0.00002 | 0.00092 | 0.00000 |
| 393.7593 | 394.5574 | 0.00734 | 0.00639 | 0.00252 |
| 393.3275 | 394.5569 | 0.00000 | 0.00016 | 0.00002 |
| 393.2728 | 394.4290 | 0.00000 | 0.00013 | 0.00001 |
| 393.2045 | 394.3903 | 0.00090 | 0.00103 | 0.00647 |
| 393.1884 | 394.0325 | 0.00000 | 0.00000 | 0.00032 |
| 393.1732 | 394.0252 | 0.00002 | 0.00049 | 0.00000 |
| 393.1062 | 394.0023 | 0.00003 | 0.00006 | 0.00000 |
| 393.0891 | 393.9639 | 0.00000 | 0.00017 | 0.00039 |
| 392.8183 | 393.9013 | 0.00967 | 0.00846 | 0.00000 |
| 392.7593 | 393.8940 | 0.00000 | 0.00010 | 0.00002 |
| 392.7261 | 393.8426 | 0.00002 | 0.00001 | 0.00000 |
| 392.6825 | 393.8197 | 0.00117 | 0.00131 | 0.00008 |
| 392.6235 | 393.8080 | 0.00000 | 0.00009 | 0.00006 |
| 392.5748 | 393.8061 | 0.00100 | 0.00132 | 0.00000 |
| 392.5280 | 393.6428 | 0.00000 | 0.00024 | 0.00000 |

Table S40: Pyridine: Unshifted RIXS data for the pump frequency at resonance with the second core excitation (core $3A'$ in Mulliken symmetry notation) calculated using different methods. RIXS cross sections for $\theta = 45°$ at the CVS-uS-EOM-CCSD and CVS-EOM-CCSD level of theory are both based on emission energies calculated at the EOM-CCSD level of theory. CVS and CVS-uS refers to a projection in the damped response solver. All calculations employed the 6-311++G** basis with additional Rydberg functions on N.

| $\omega_{em}$/eV | | $\sigma^{\mathrm{RIXS}}_{45°}$/a.u. | | |
|---|---|---|---|---|
| CCSD | CC2 | CVS-uS-EOM-CCSD | CVS-EOM-CCSD | CVS-uS-EOM-CC2 |
| 399.4296 | 398.0663 | 0.00019 | 0.00011 | 0.00054 |
| 399.3502 | 397.7999 | 0.00000 | 0.00001 | 0.00001 |
| 398.9779 | 397.7882 | 0.00001 | 0.00001 | 0.00000 |
| 397.9003 | 397.0489 | 0.00002 | 0.00044 | 0.00001 |
| 397.8995 | 396.5267 | 0.00002 | 0.0009 | 0.00000 |
| 397.785 | 396.4734 | 0.00001 | 0.00016 | 0.00074 |
| 397.3531 | 396.4728 | 0.00006 | 0.0002 | 0.00002 |
| 397.2984 | 396.3449 | 0.00000 | 0.00015 | 0.00001 |
| 397.2301 | 396.3063 | 0.0019 | 0.00199 | 0.00005 |
| 397.2141 | 395.9485 | 0.00000 | 0.00000 | 0.00004 |
| 397.1988 | 395.9414 | 0.00026 | 0.00066 | 0.00001 |
| 397.1319 | 395.9185 | 0.00024 | 0.00023 | 0.00001 |
| 397.1147 | 395.8802 | 0.00000 | 0.00017 | 0.00007 |
| 396.844 | 395.8173 | 0.0001 | 0.00026 | 0.00000 |
| 396.7849 | 395.8099 | 0.00000 | 0.00012 | 0.00004 |
| 396.7517 | 395.7585 | 0.00001 | 0.00000 | 0.00000 |
| 396.7079 | 395.7357 | 0.00000 | 0.00022 | 0.00001 |
| 396.6491 | 395.724 | 0.00001 | 0.00014 | 0.00001 |
| 396.6004 | 395.7221 | 0.00007 | 0.00061 | 0.00000 |
| 396.5536 | 395.5588 | 0.00001 | 0.00026 | 0.00000 |

Table S41: Pyridine: Unshifted nonresonant (XES) data at the Nitrogen $K$-edge calculated using different methods. All calculations employed the 6-311++G** basis with additional Rydberg functions on N.

| $\omega_{em}$/eV | | $f_{osc}$ | |
|---|---|---|---|
| CCSD | CC2 | EOM-CCSD | EOM-CC2 |
| 397.1485 | 396.0404 | 0.03456 | 0.03739 |
| 397.0568 | 395.1555 | 0.00000 | 0.00000 |
| 396.3471 | 394.5316 | 0.01904 | 0.01956 |
| 393.9024 | 392.4991 | 0.00747 | 0.00822 |
| 393.1568 | 391.7691 | 0.01270 | 0.01297 |
| 392.7334 | 391.4161 | 0.00490 | 0.00426 |
| 391.9707 | 390.5742 | 0.00061 | 0.00061 |
| 390.7810 | 389.7628 | 0.01340 | 0.01475 |
| 390.6047 | 389.0661 | 0.00012 | 0.00009 |
| 389.0604 | 387.7067 | 0.00170 | 0.00150 |
| 387.9771 | 385.3961 | 0.00000 | 0.00000 |
| 387.2683 | 385.2941 | 0.00005 | 0.00000 |
| 387.0686 | 385.2881 | 0.00036 | 0.00000 |
| 386.8784 | 385.1847 | -0.00004 | 0.00000 |
| 386.3167 | 385.1072 | 0.00005 | 0.00000 |
| 386.2636 | 385.1063 | 0.00776 | 0.00000 |
| 385.8811 | 385.0938 | 0.00000 | 0.00000 |
| 385.7657 | 385.0321 | 0.00009 | 0.00808 |

# References

(1) Prince, K. C.; Richter, R.; de Simone, M.; Alagia, M.; Coreno, M. Near Edge X-ray Absorption Spectra of Some Small Polyatomic Molecules. *J. Phys. Chem. A* **2003**, *107*, 1955–1963.

(2) Bodeur, S.; Esteva, J. M. Photoabsorption spectra of $H_2S$, $CH_3SH$ and $SO_2$ near the sulfur *K* edge. *J. Chem. Phys.* **1985**, *100*, 415–427.

(3) Carbone, J. P.; Cheng, L.; Myhre, R. H.; Matthews, D.; Koch, H.; Coriani, S. In *State of The Art of Molecular Electronic Structure Computations: Correlation Methods, Basis Sets and More*; Ancarani, L. U., Hoggan, P. E., Eds.; Advances in Quantum Chemistry; Academic Press, 2019; Vol. 79; pp 241–261.

(4) Turci, C. C.; Urquhart, S. G.; Hitchcock, A. P. Inner-shell excitation spectroscopy of aniline, nitrobenzene, and nitroanilines. *Can. J. Chem.* **1996**, *74*, 851–869.

(5) Meyer, F.; Blum, M.; Benkert, A.; Hauschild, D.; Jeyachandran, Y. L.; Wilks, R. G.; Yang, W.; Bär, M.; Reinert, F.; Heske, C.; Zharnikov, M.; Weinhardt, L. Site-specific electronic structure of imidazole and imidazolium in aqueous solutions. *Phys. Chem. Chem. Phys.* **2018**, *20*, 8302–8310.

(6) Baiardi, A.; Mendolicchio, M.; Barone, V.; Fronzoni, G.; Cardenas Jimenez, G. A.; Stener, M.; Grazioli, C.; de Simone, M.; Coreno, M. Vibrationally resolved NEXAFS at C and N K-edges of pyridine, 2-fluoropyridine and 2,6-difluoropyridine: A combined experimental and theoretical assessment. *J. Chem. Phys.* **2015**, *143*, 204102.

(7) Arimura, M.; Yoshikawa, Y. Ionization Efficiency and Ionization Energy of Cyclic Compounds by Electron Impact. *J. Mass Spectrom. Soc. Jpn.* **1984**, *32*, 375–380.

(8) Brown, R. S.; Tse, A.; Vederas, J. C. Photoelectron-determined core binding energies and predicted gas-phase basicities for the 2-hydroxypyridine $\rightleftharpoons$ 2-pyridone system. *J. Am. Chem. Soc.* **1980**, *102*, 1174–1176.
